# Supplementary material for: InsQABench: Benchmarking Chinese Insurance Domain Question Answering with Large Language Models
Source: arXiv:2501.10943 source file (2025-01-19)

Question Types in Commonsense QA Dataset

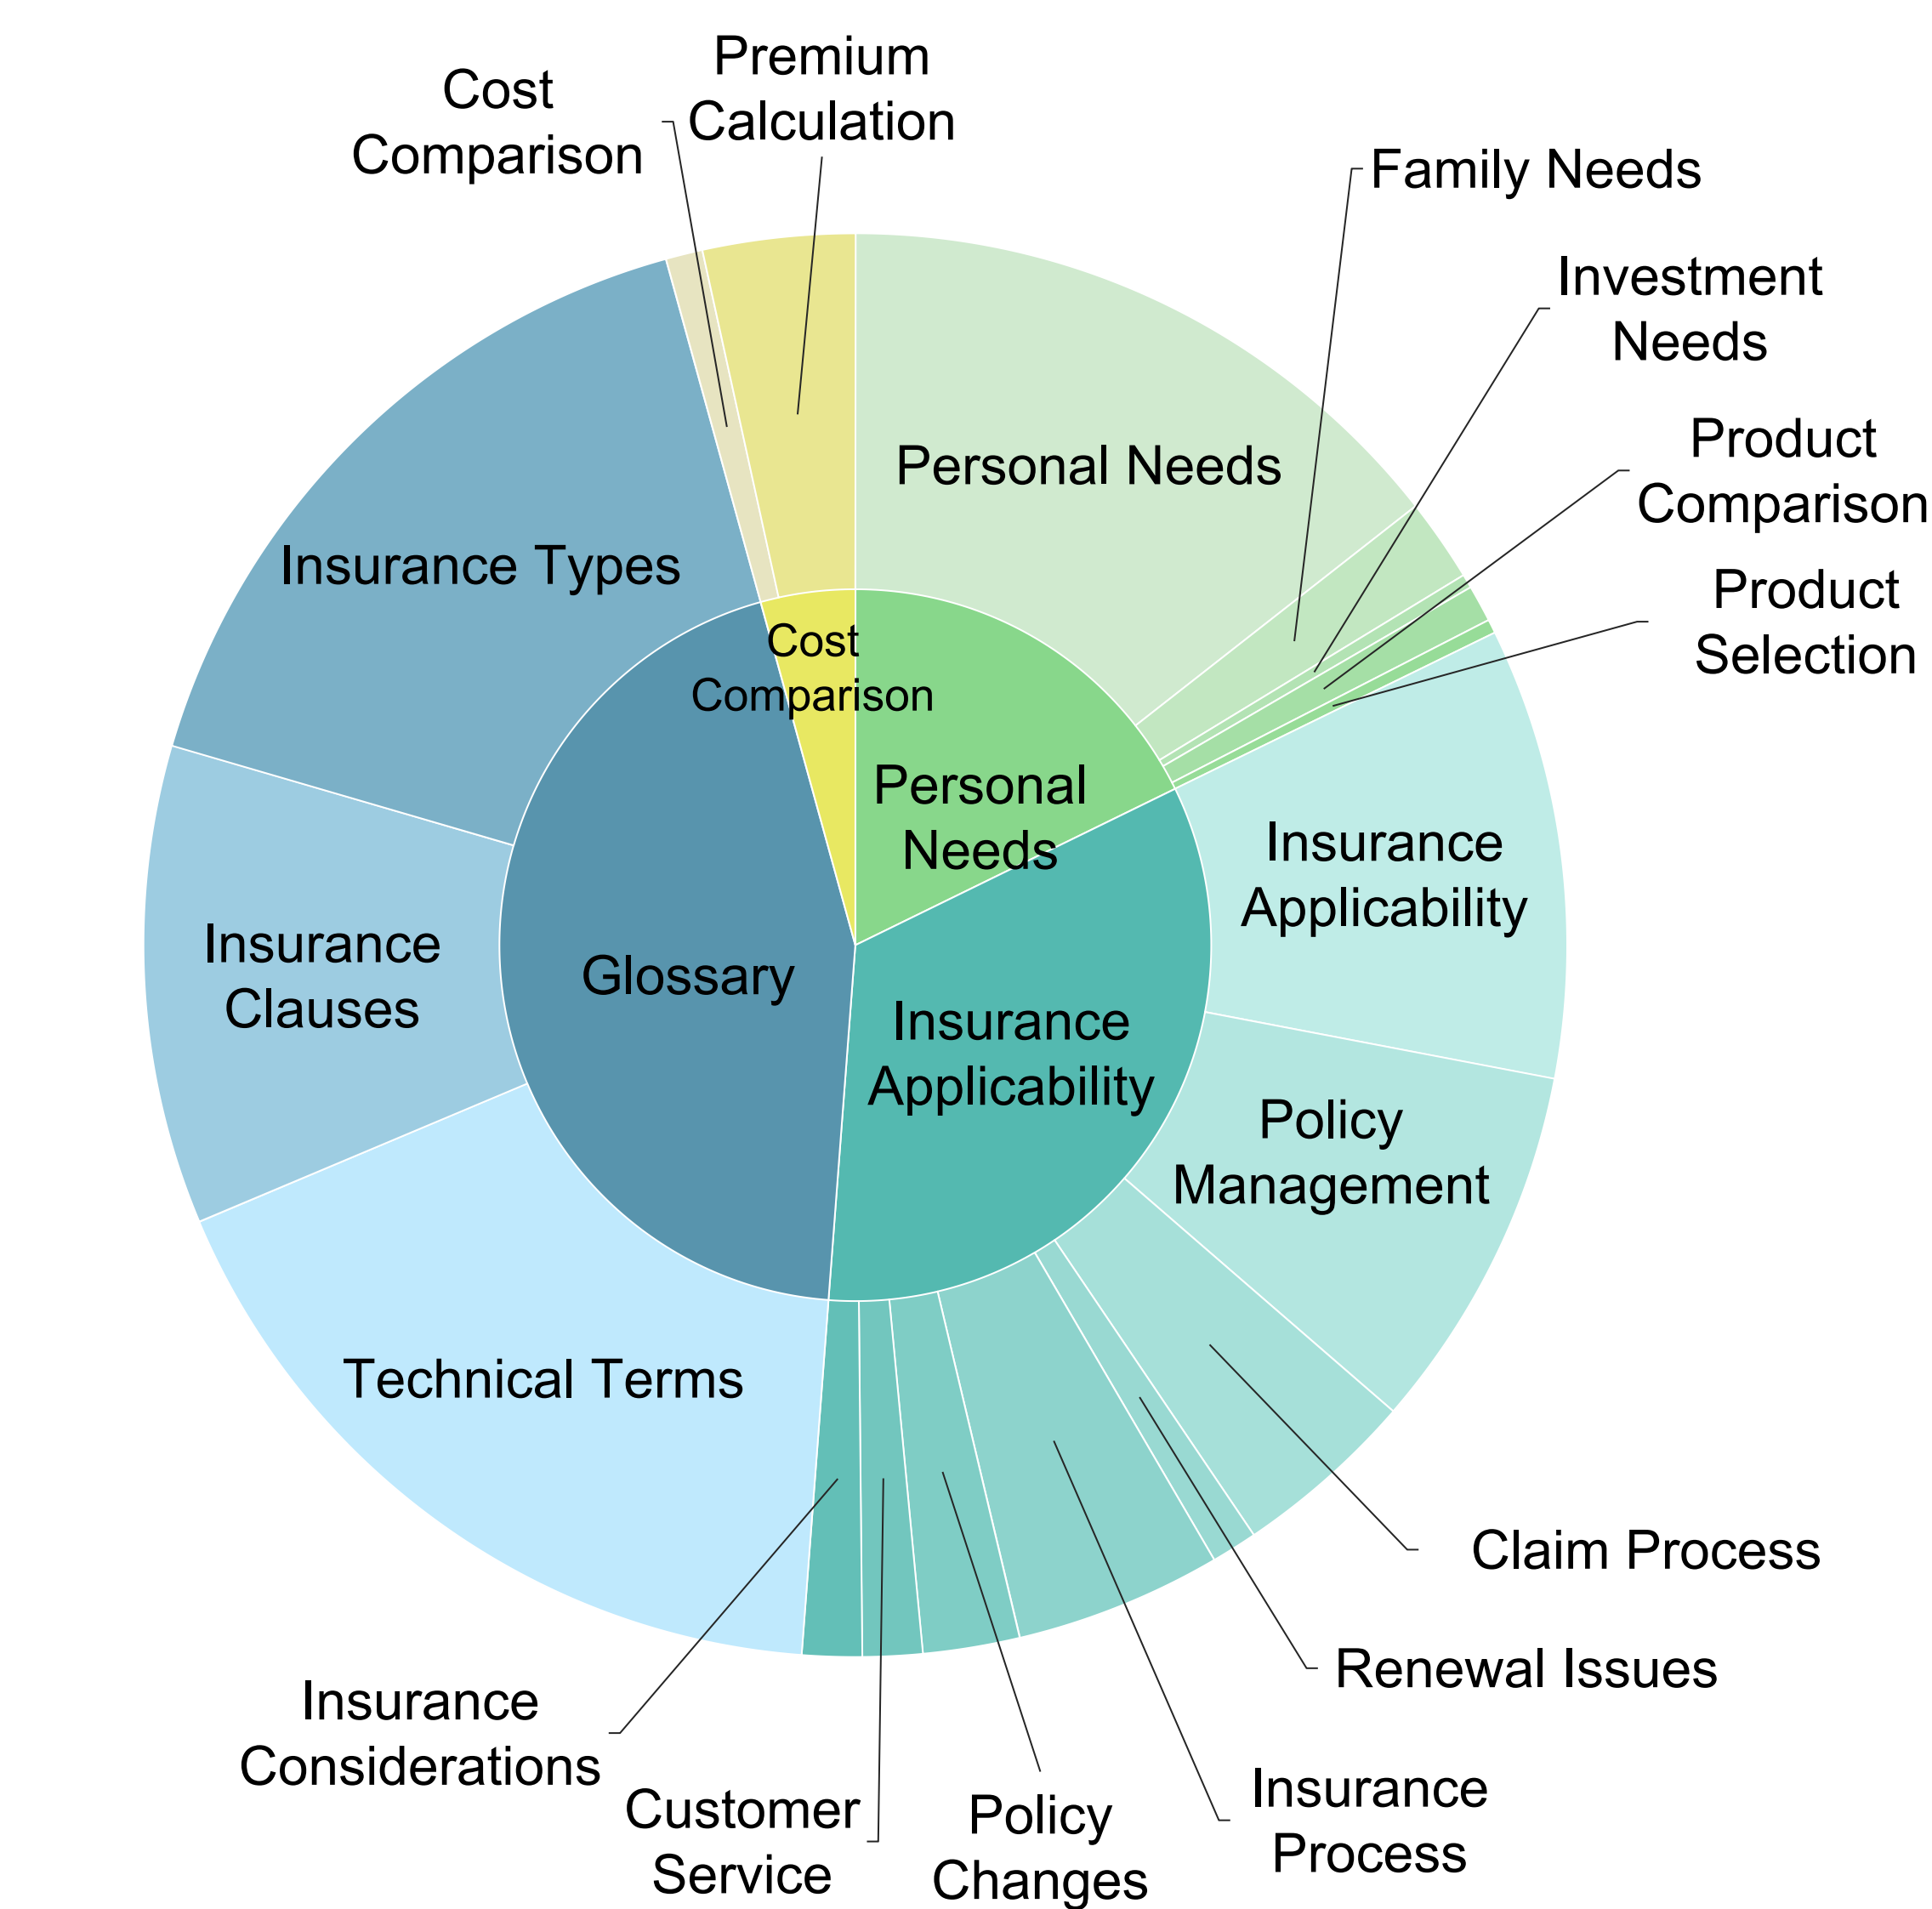

Topics in Commonsense QA Dataset

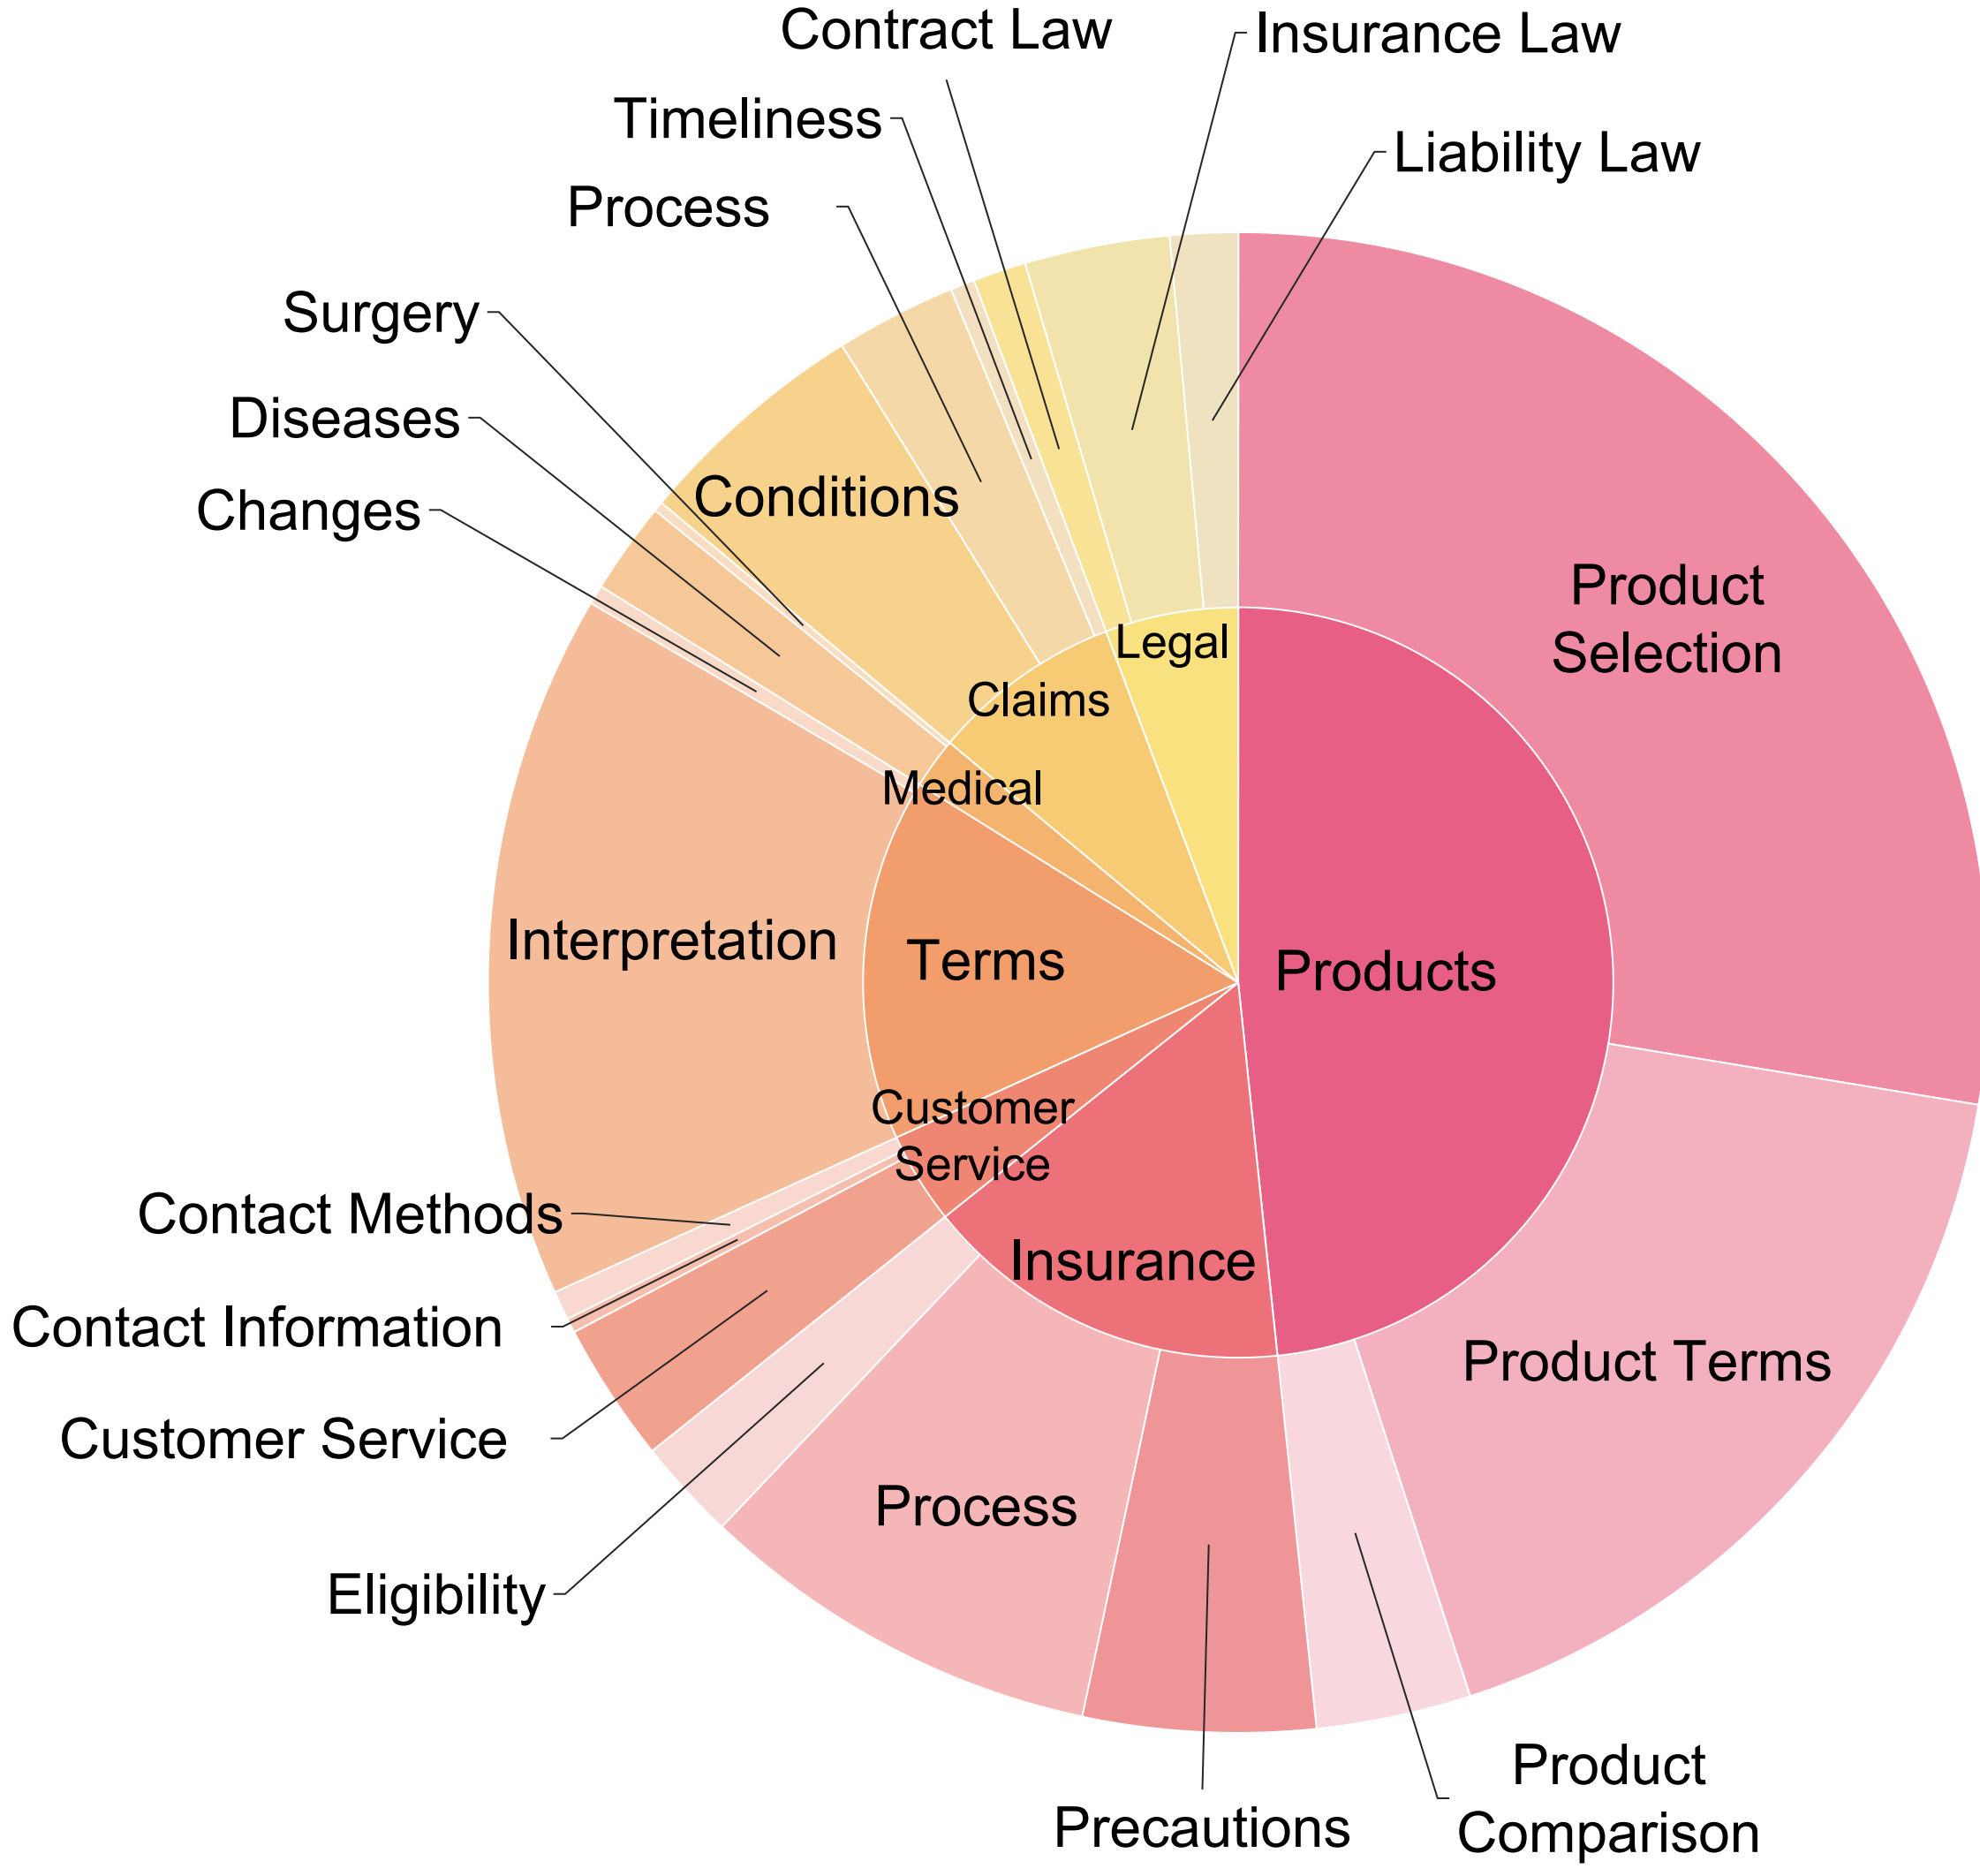

Question Types in Database QA Dataset

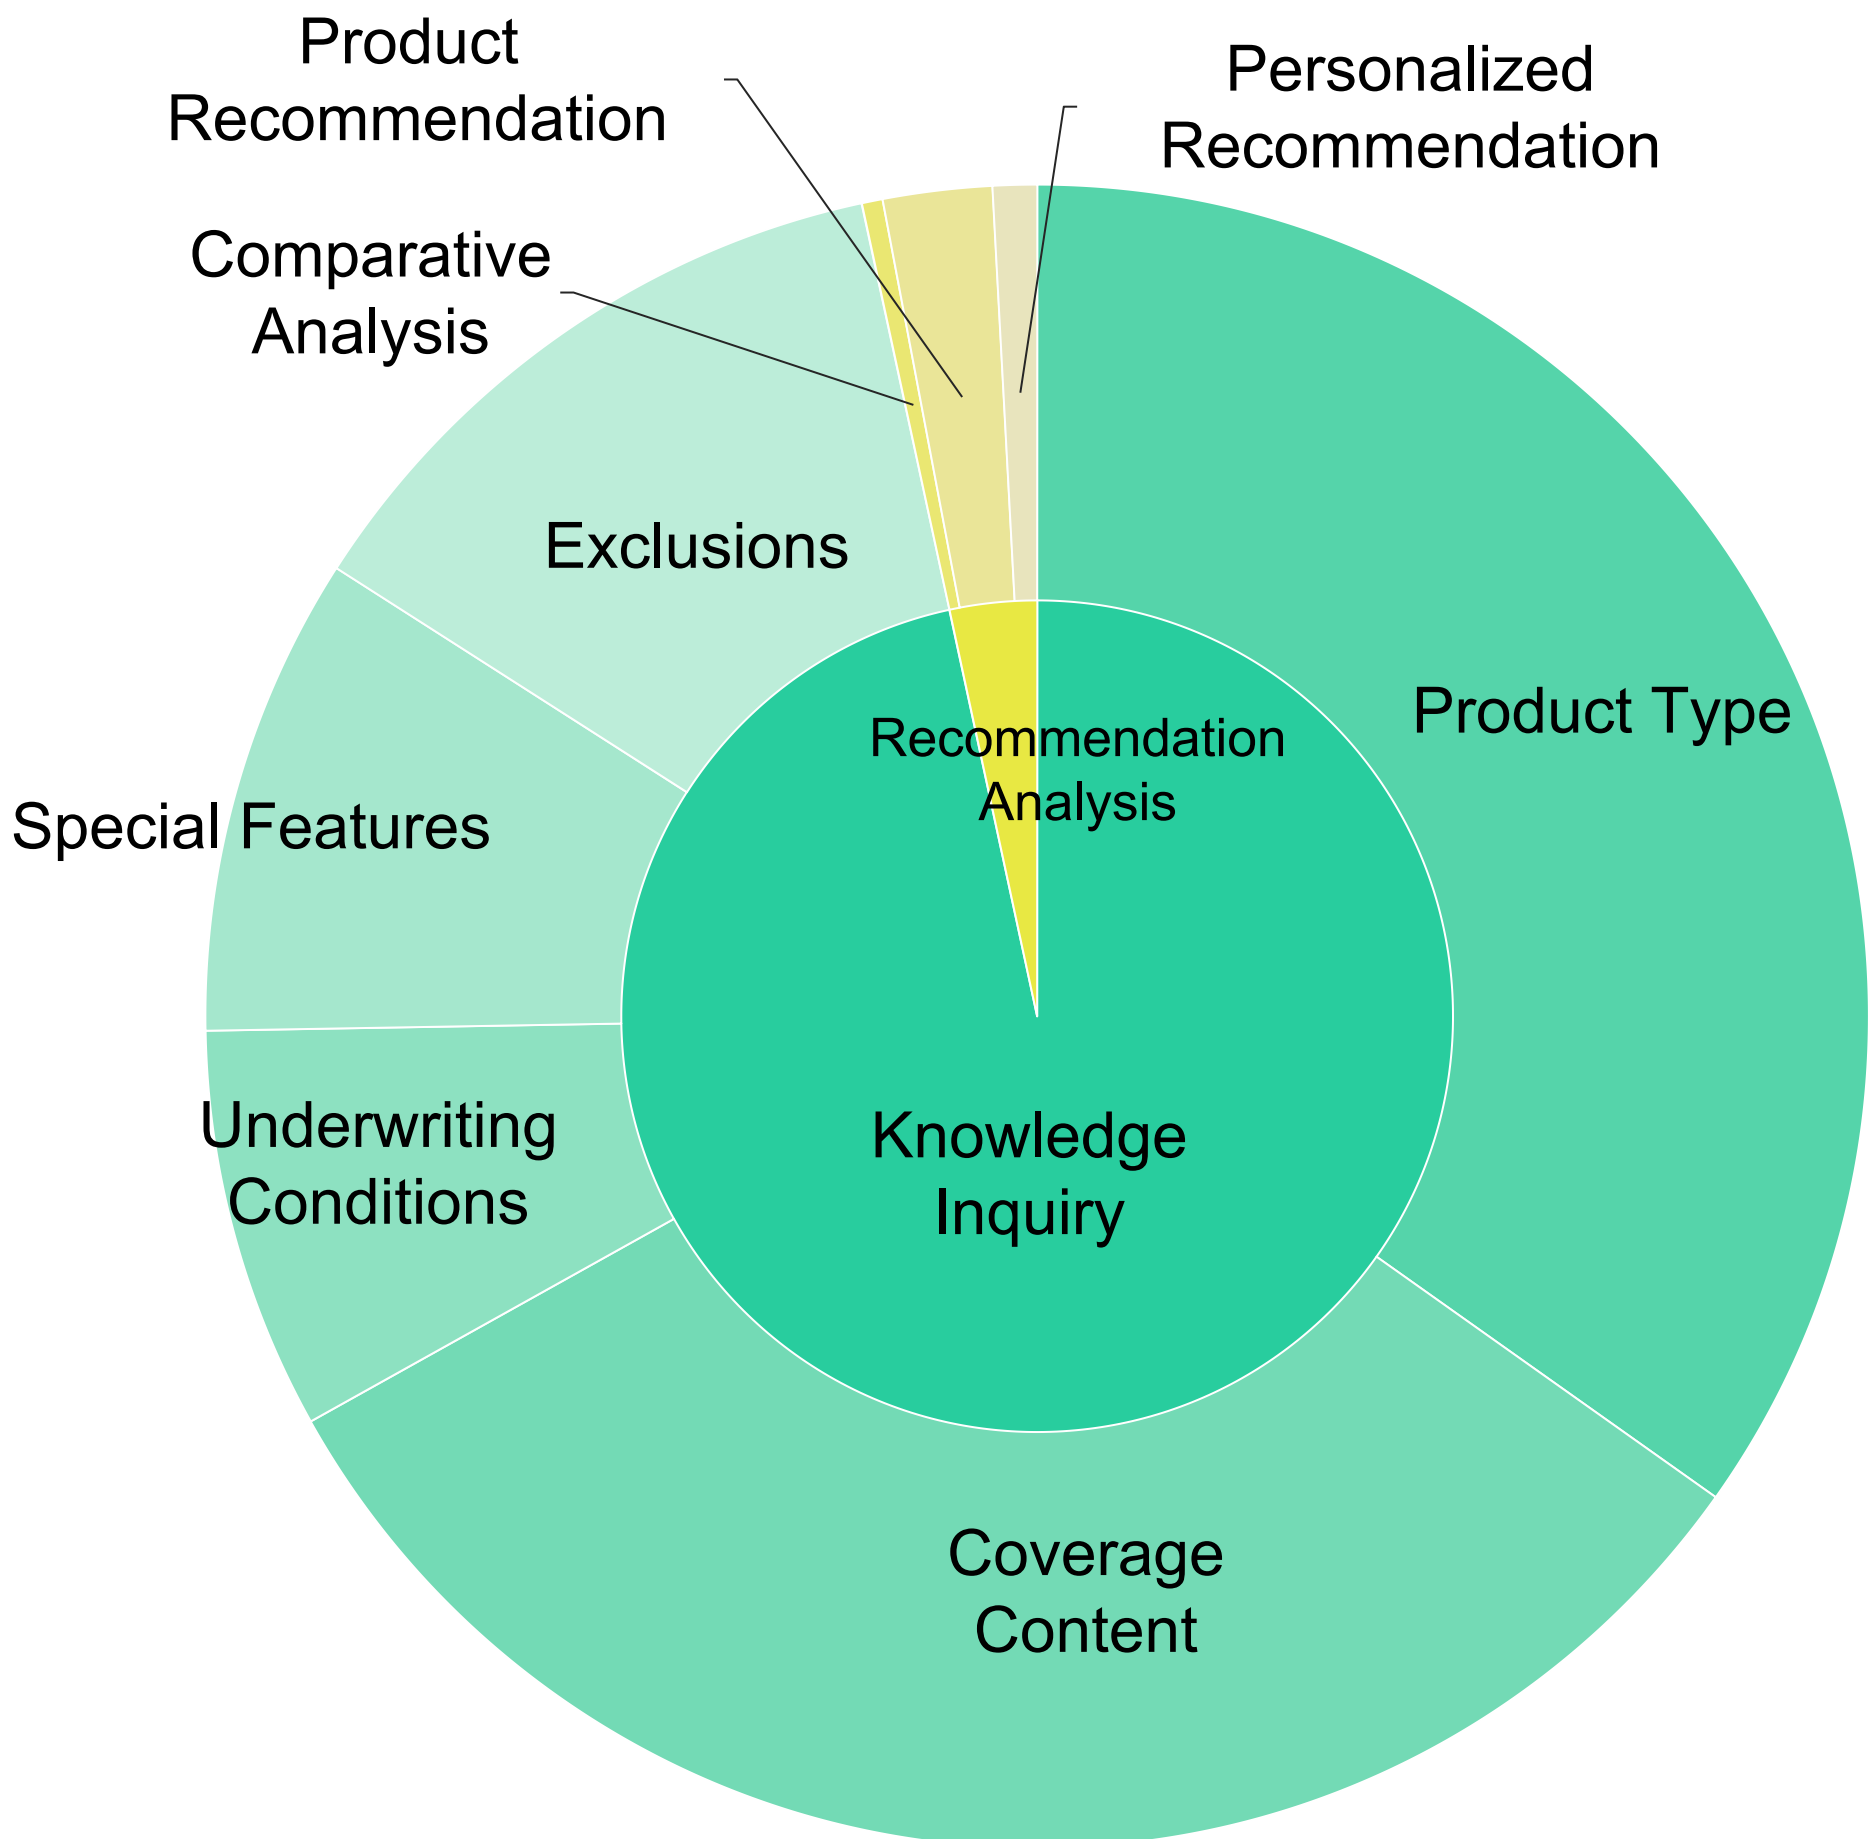

Topics in Database QA Dataset

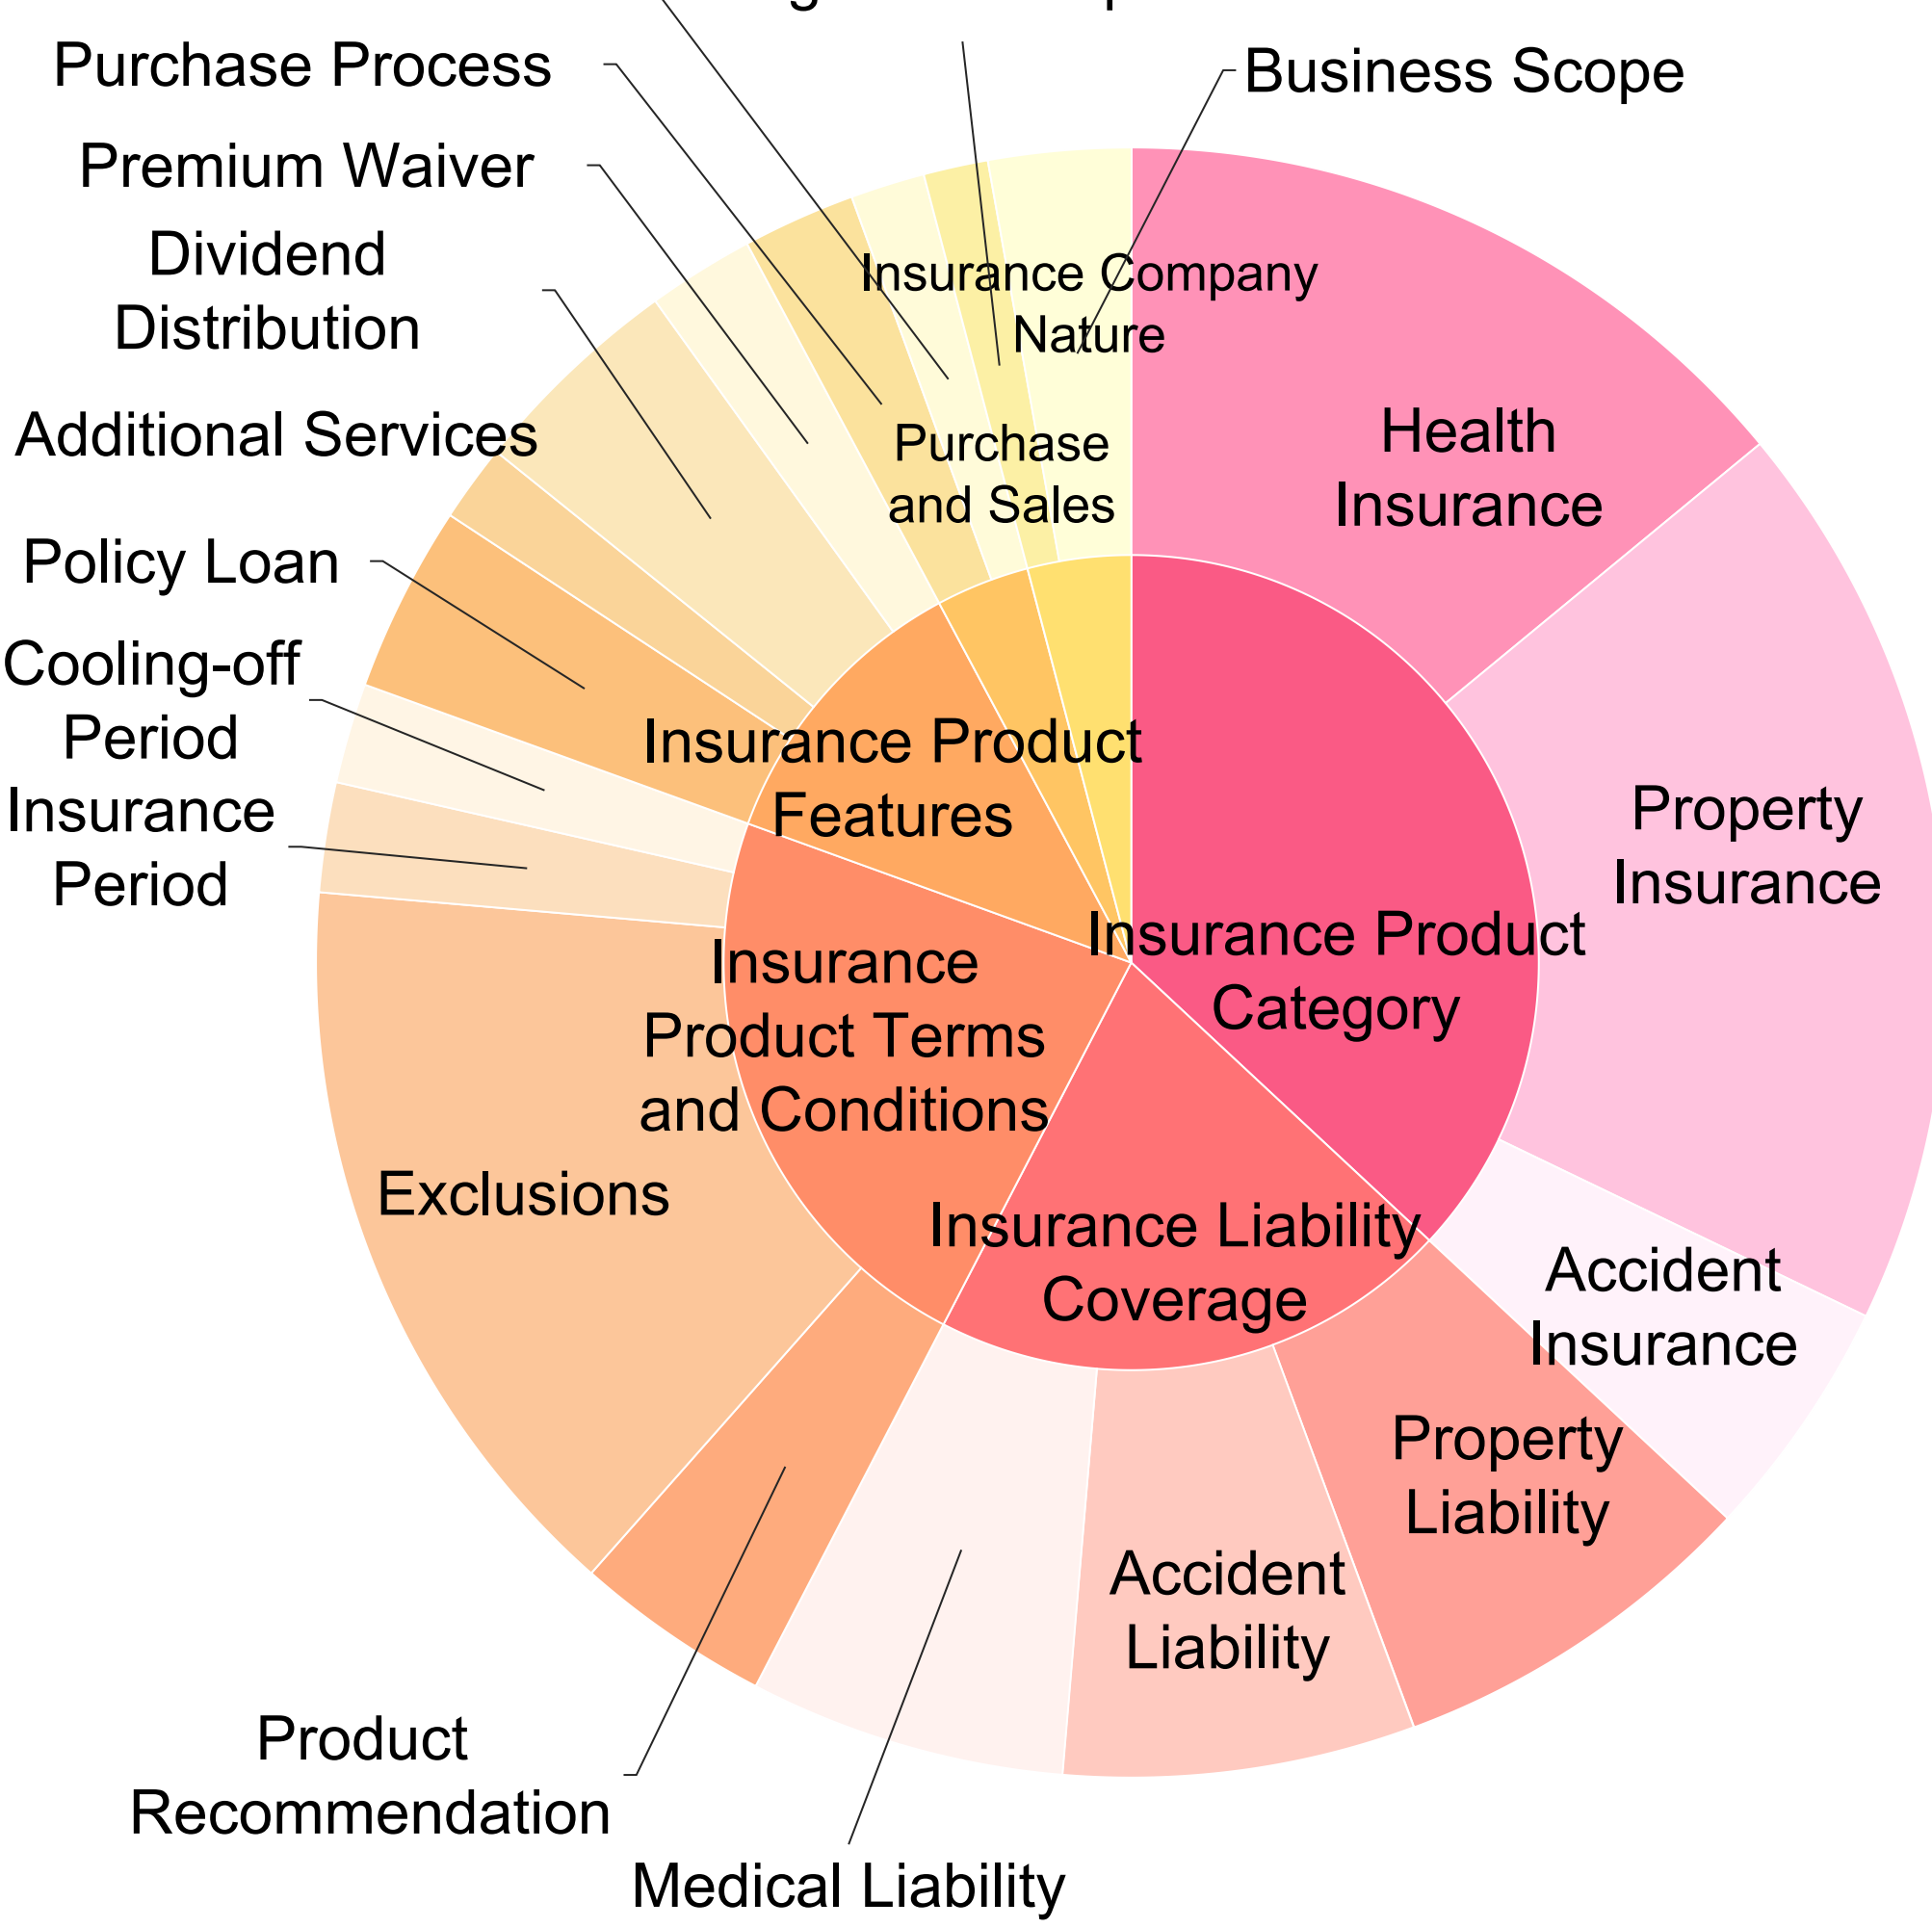

Question Types in Clause QA Dataset

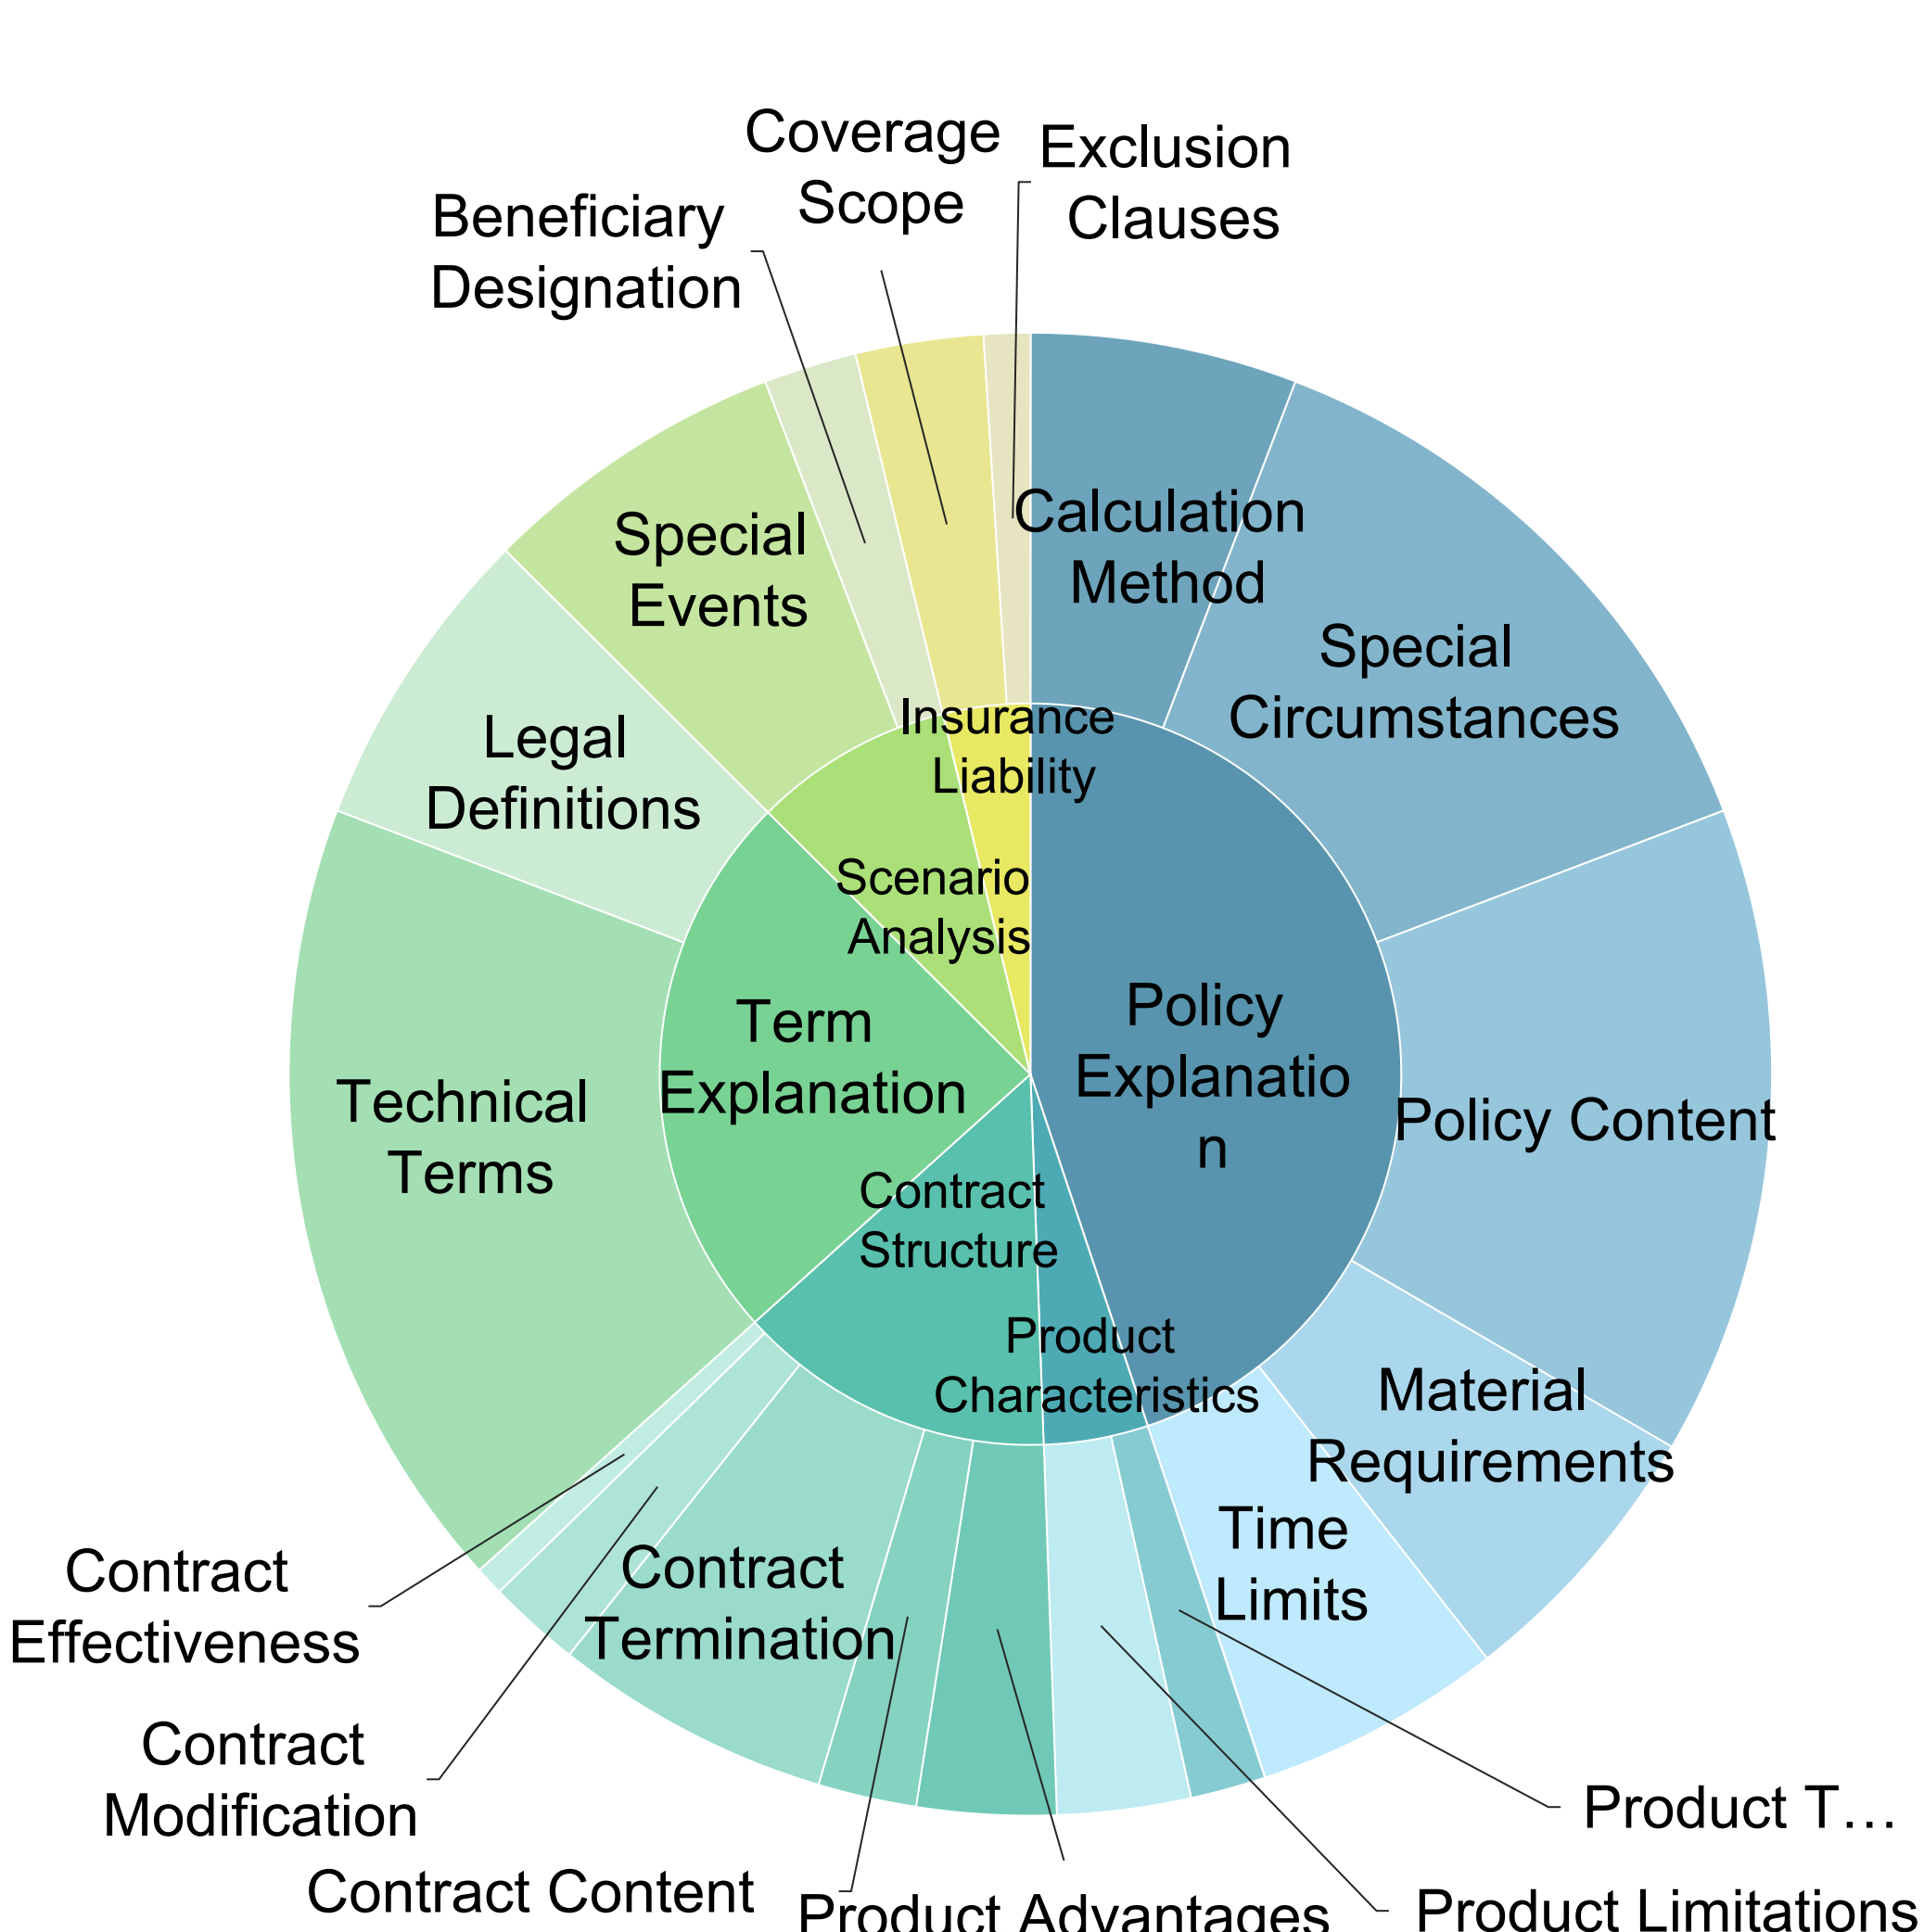

Topics in Clause QA Dataset

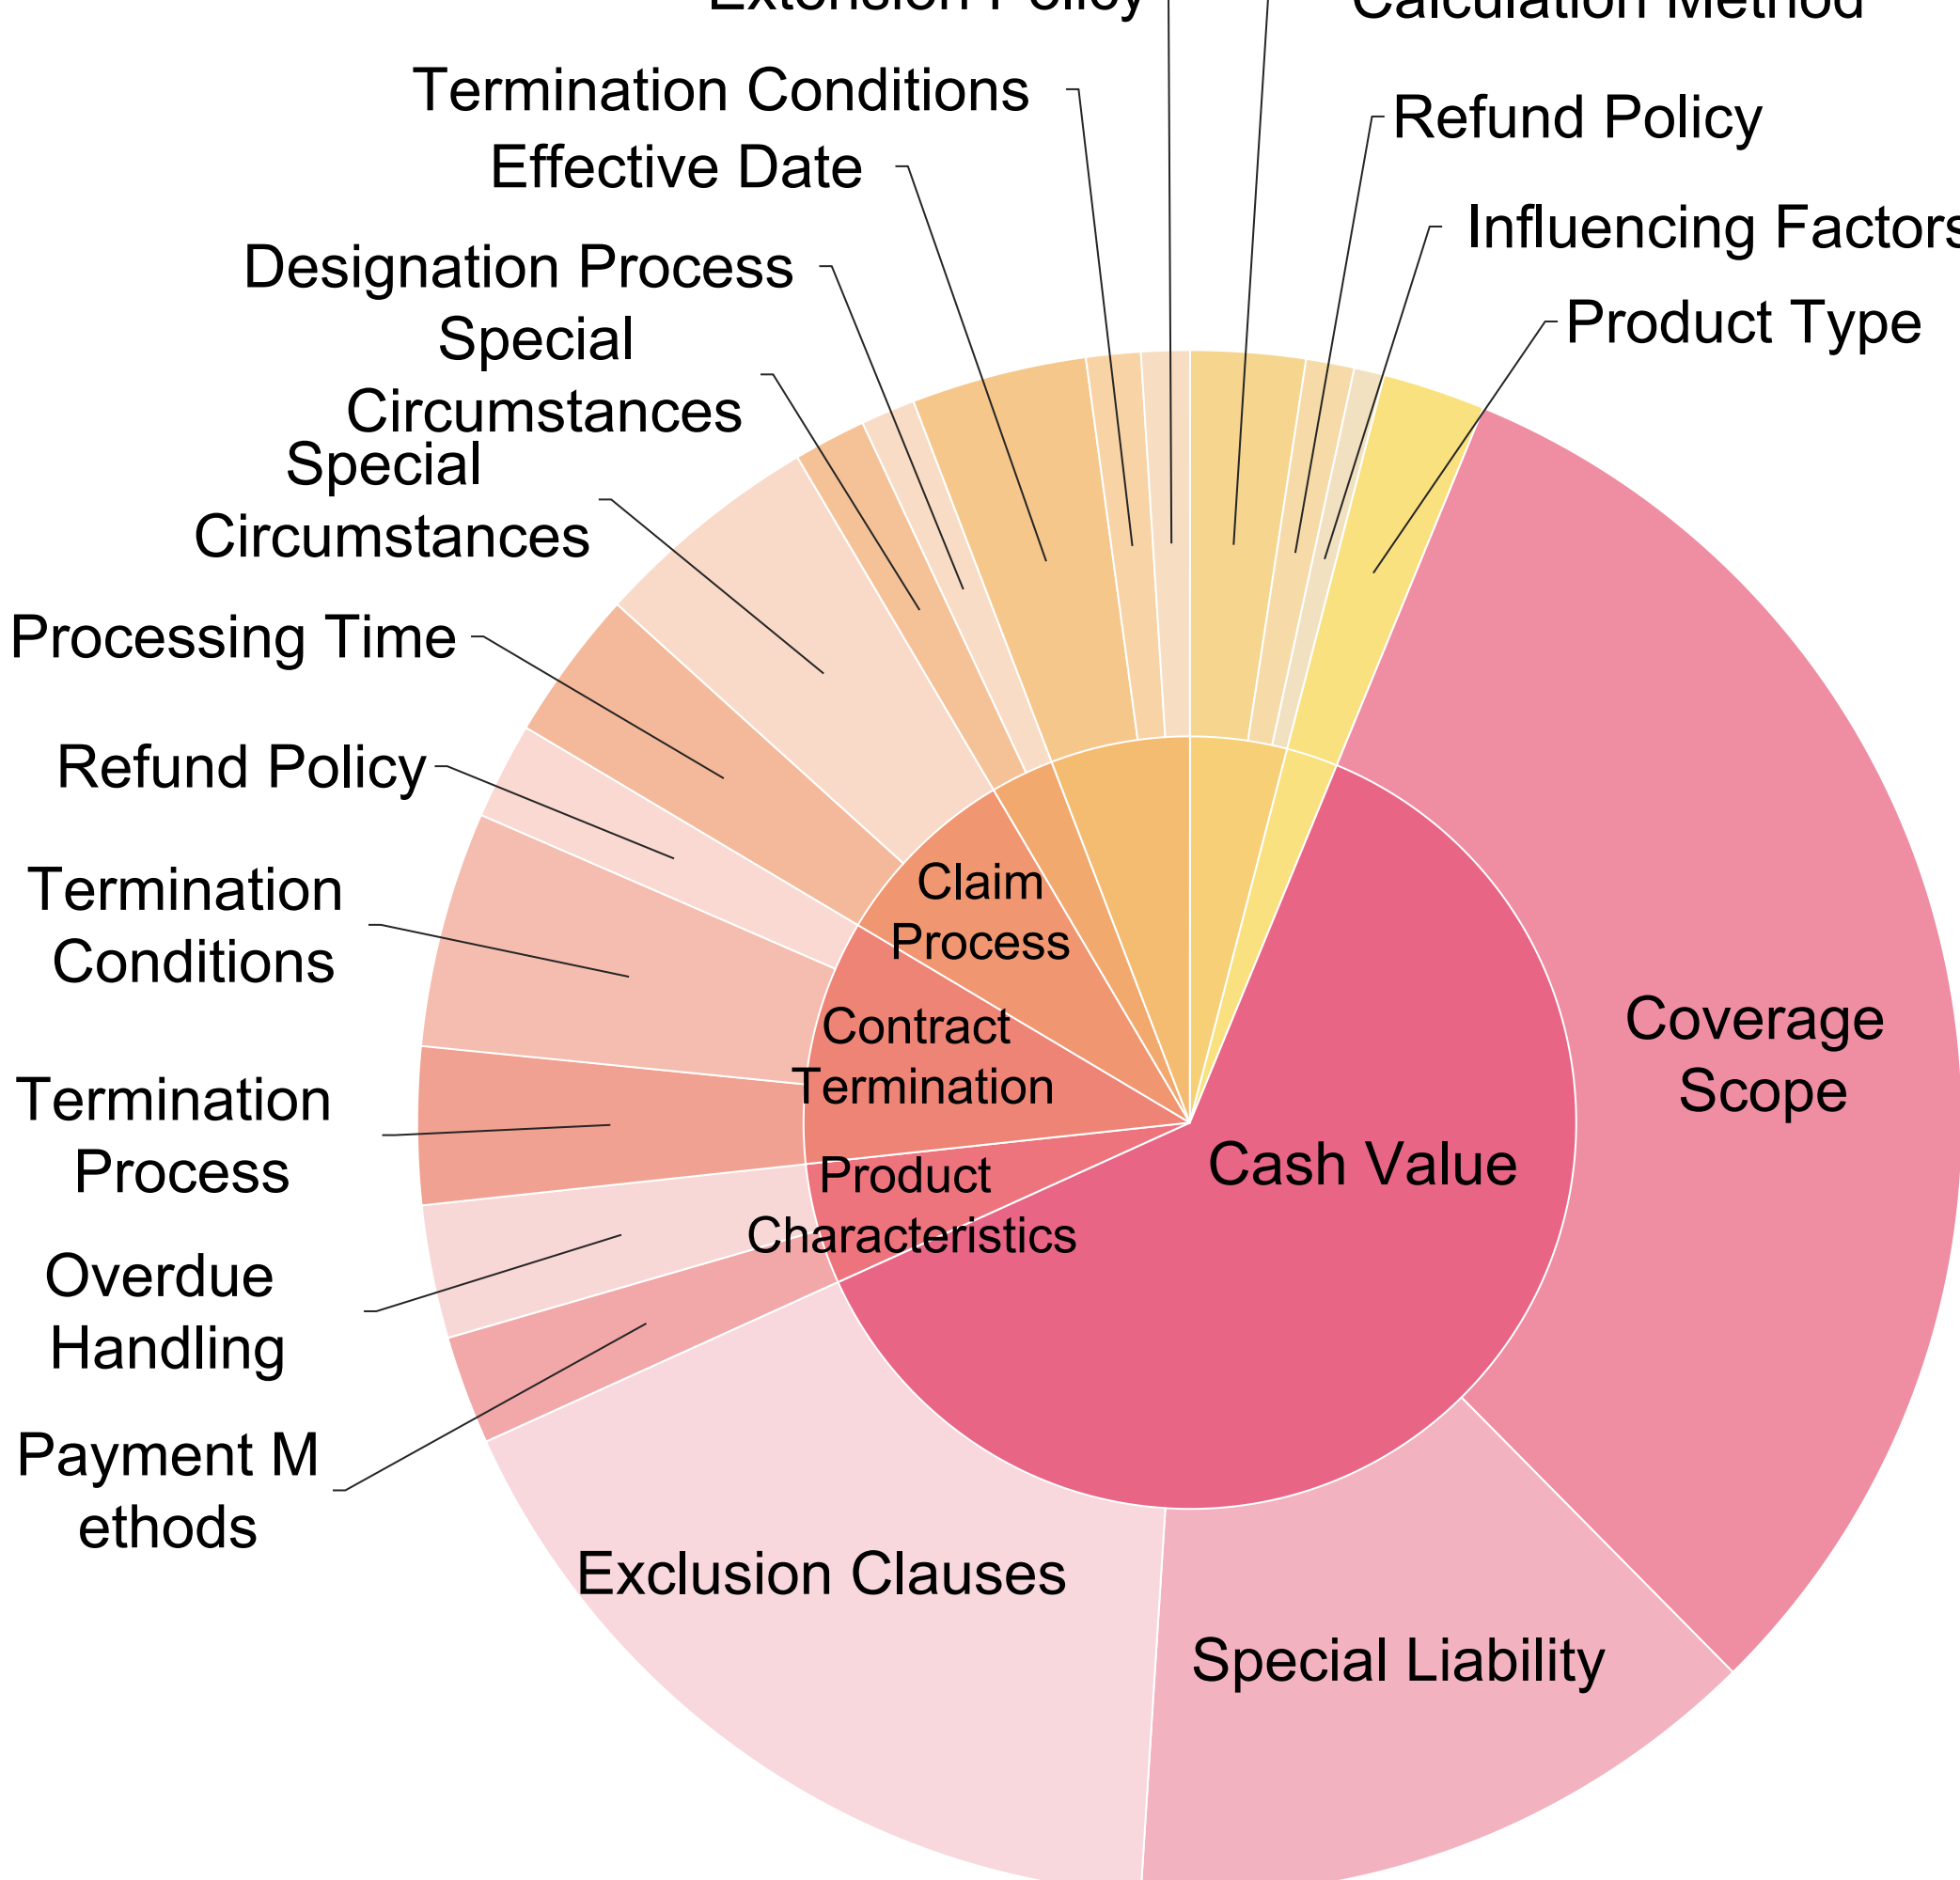



Question Types in Clause QA Dataset

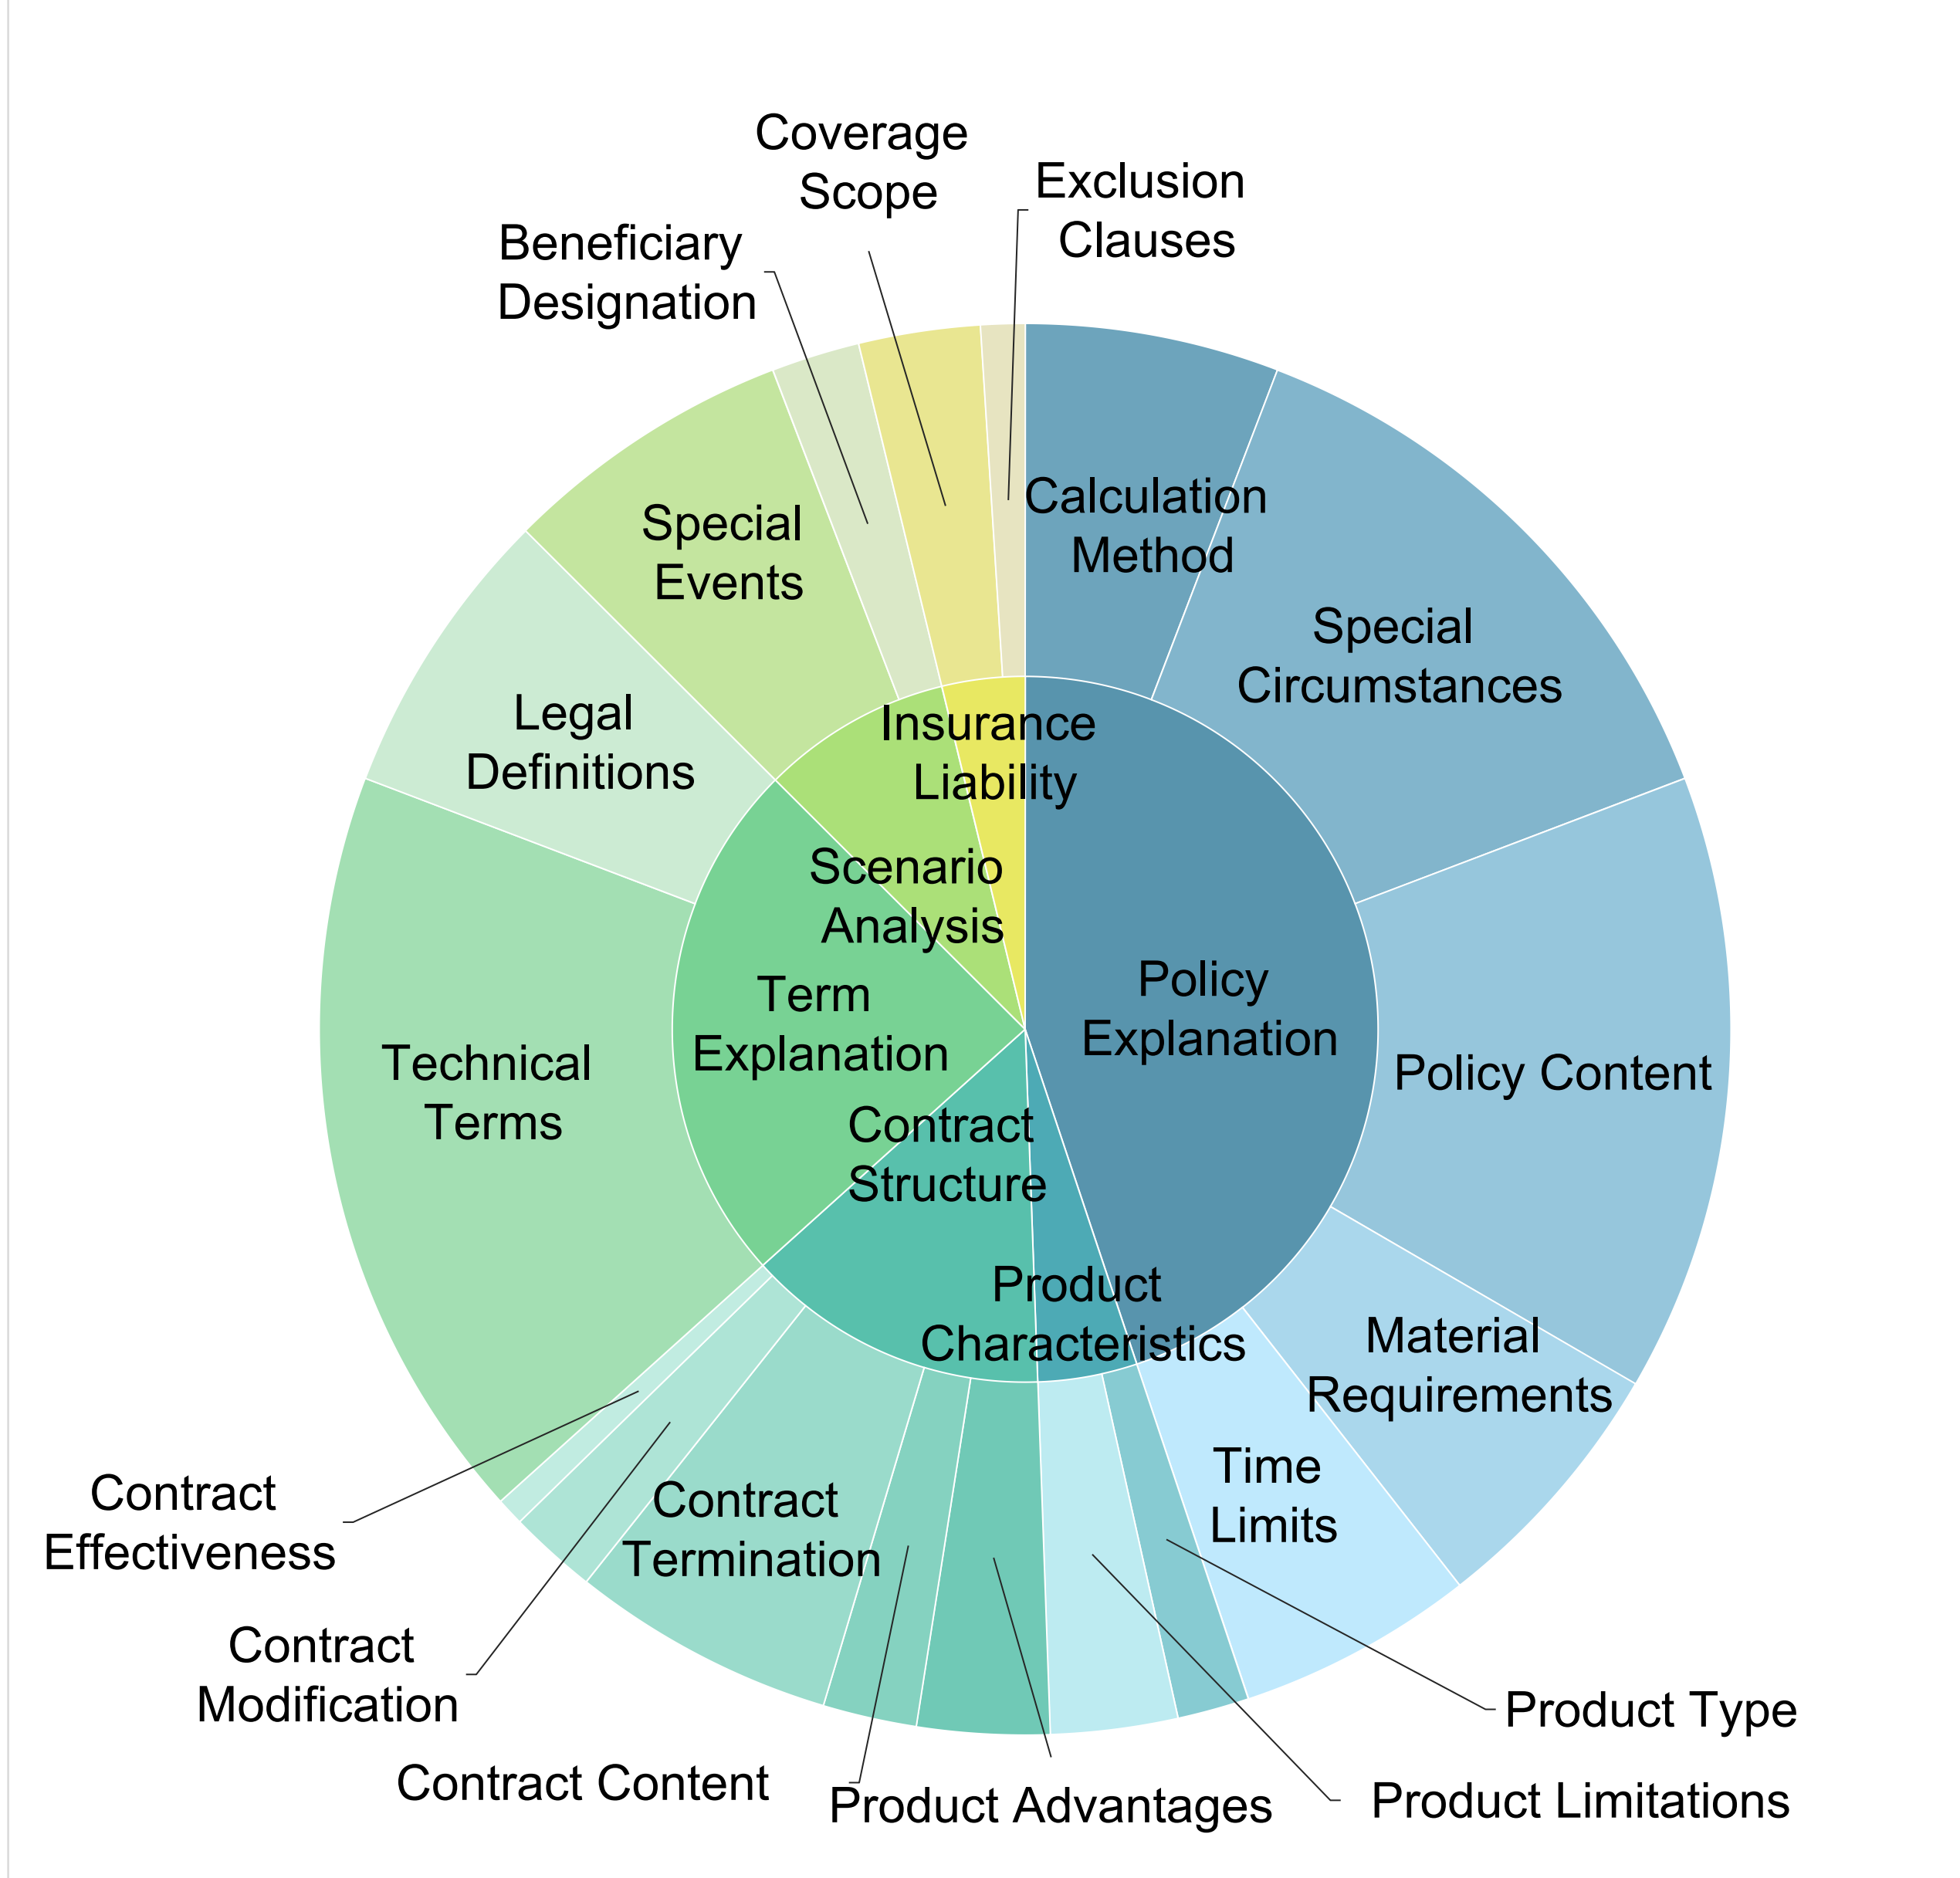

Topics in Clause QA Dataset

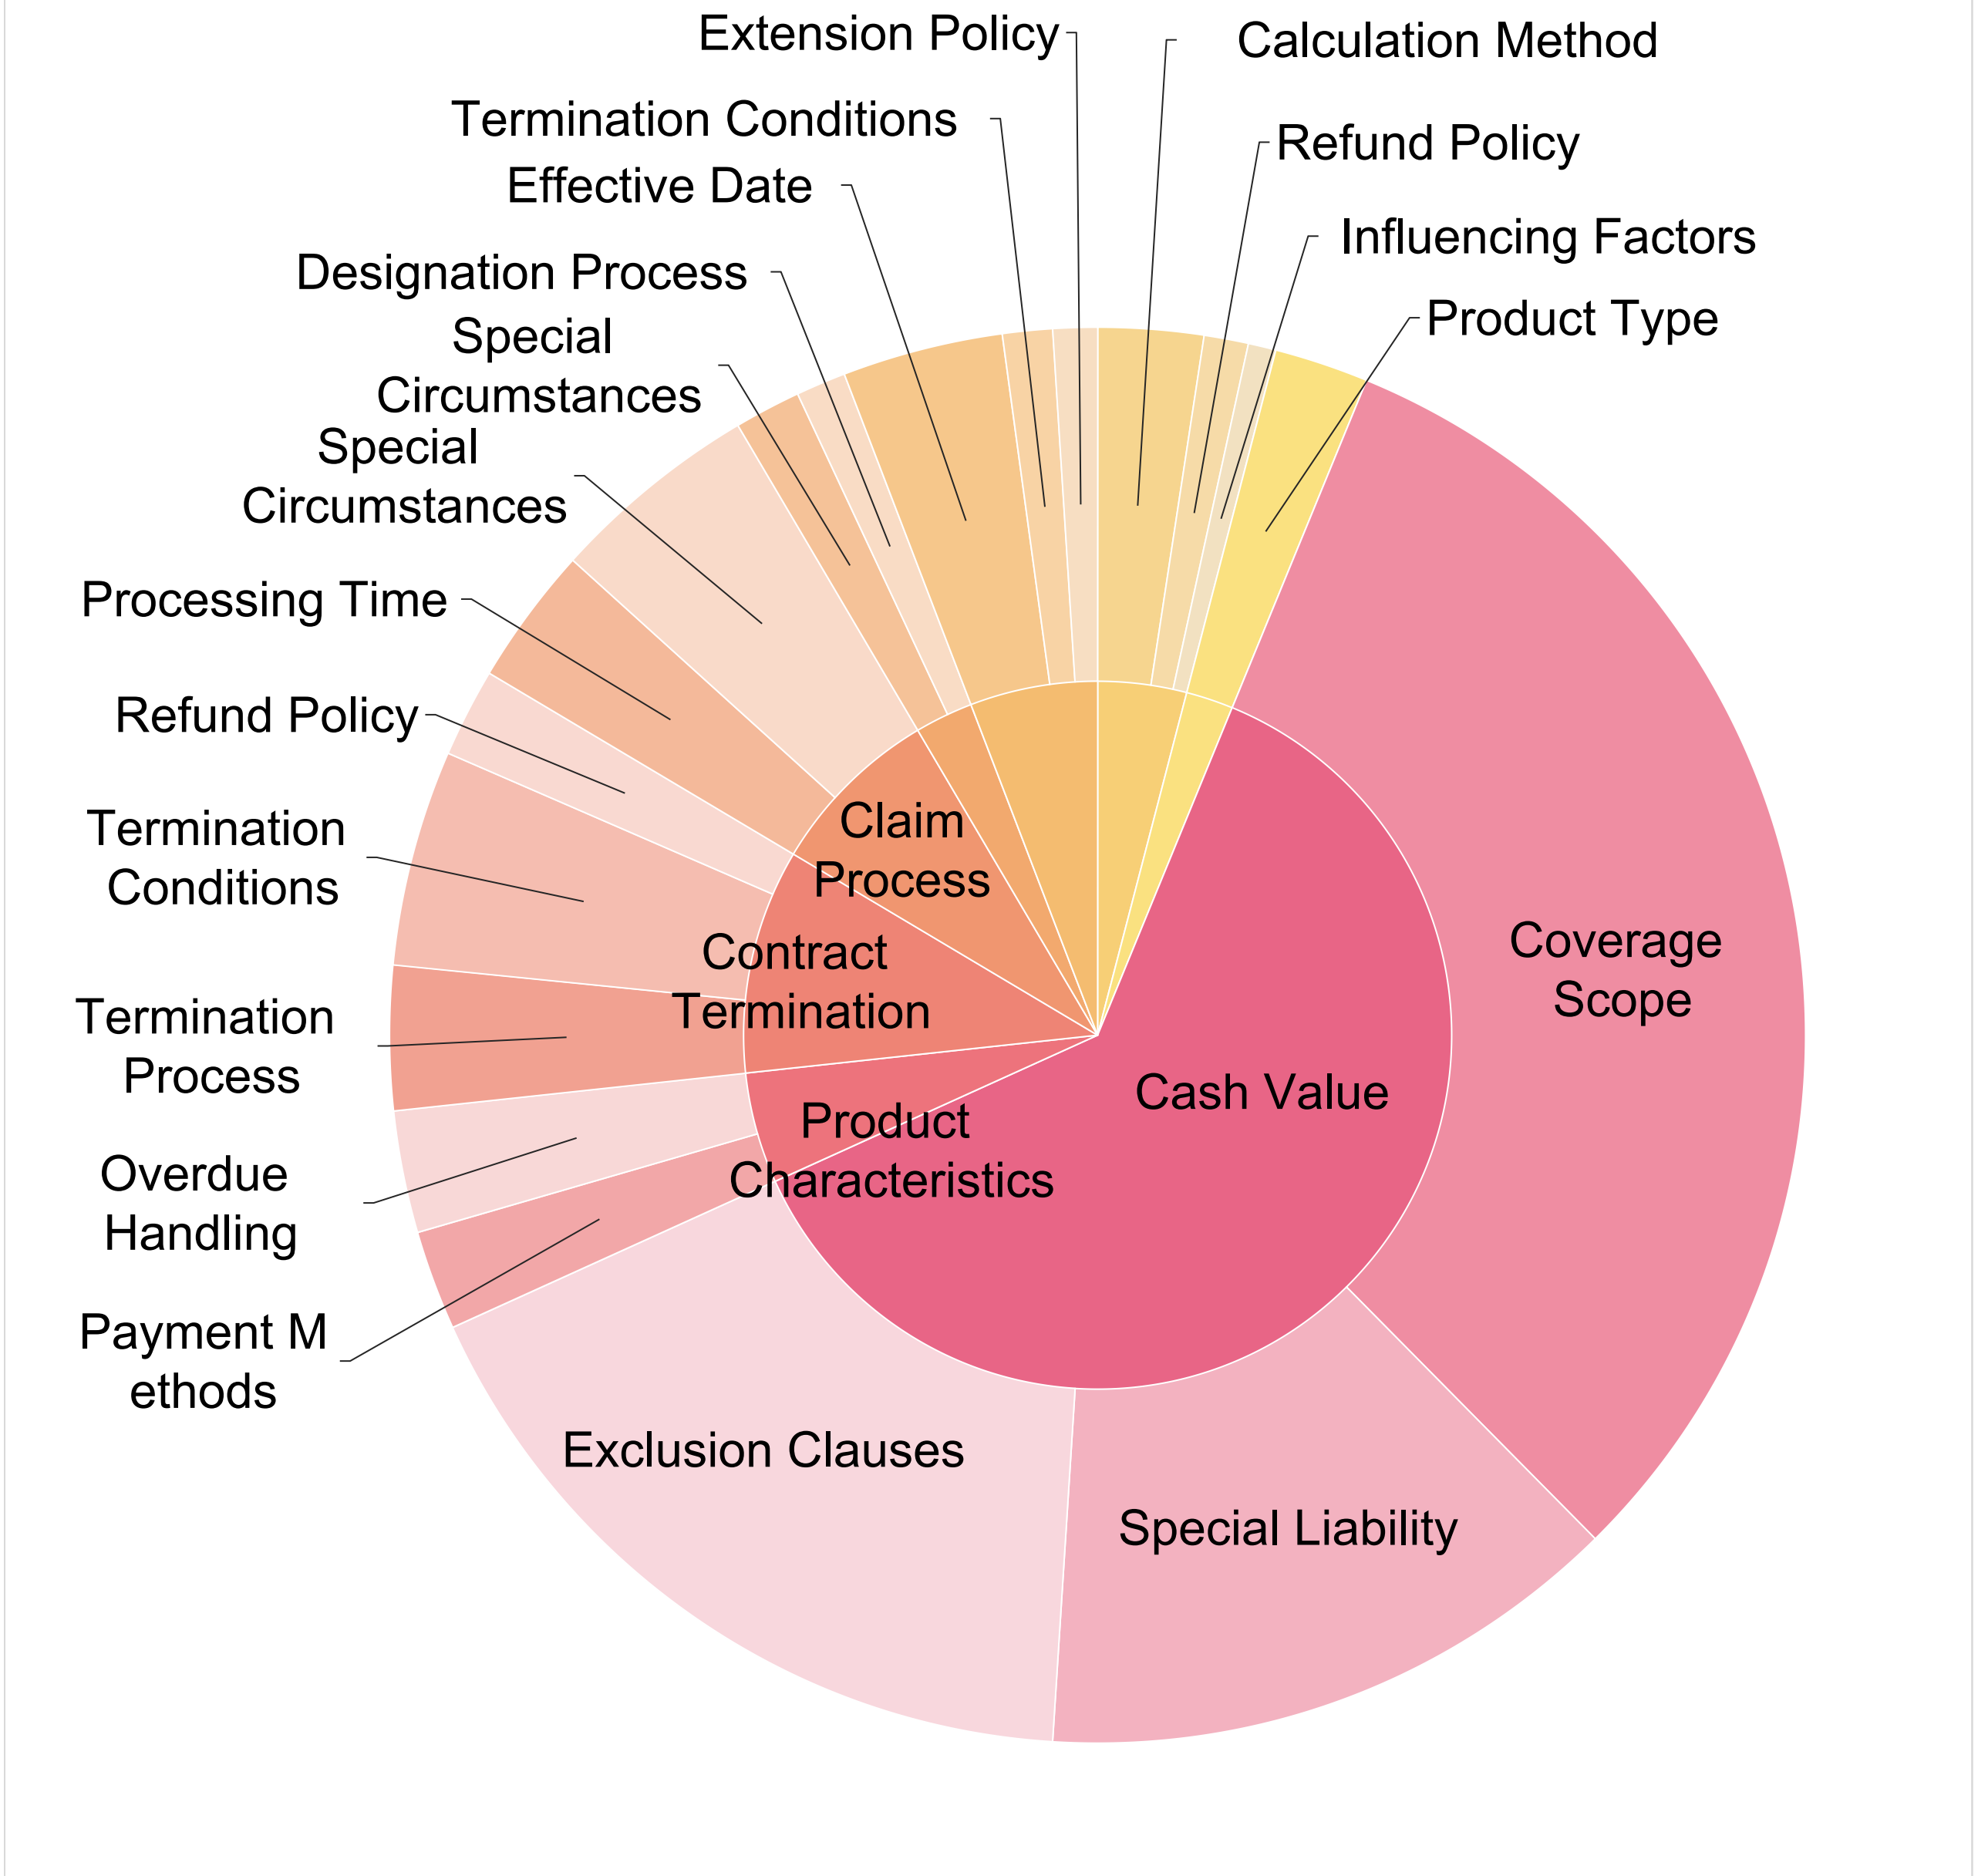

Question Types in Database QA Dataset

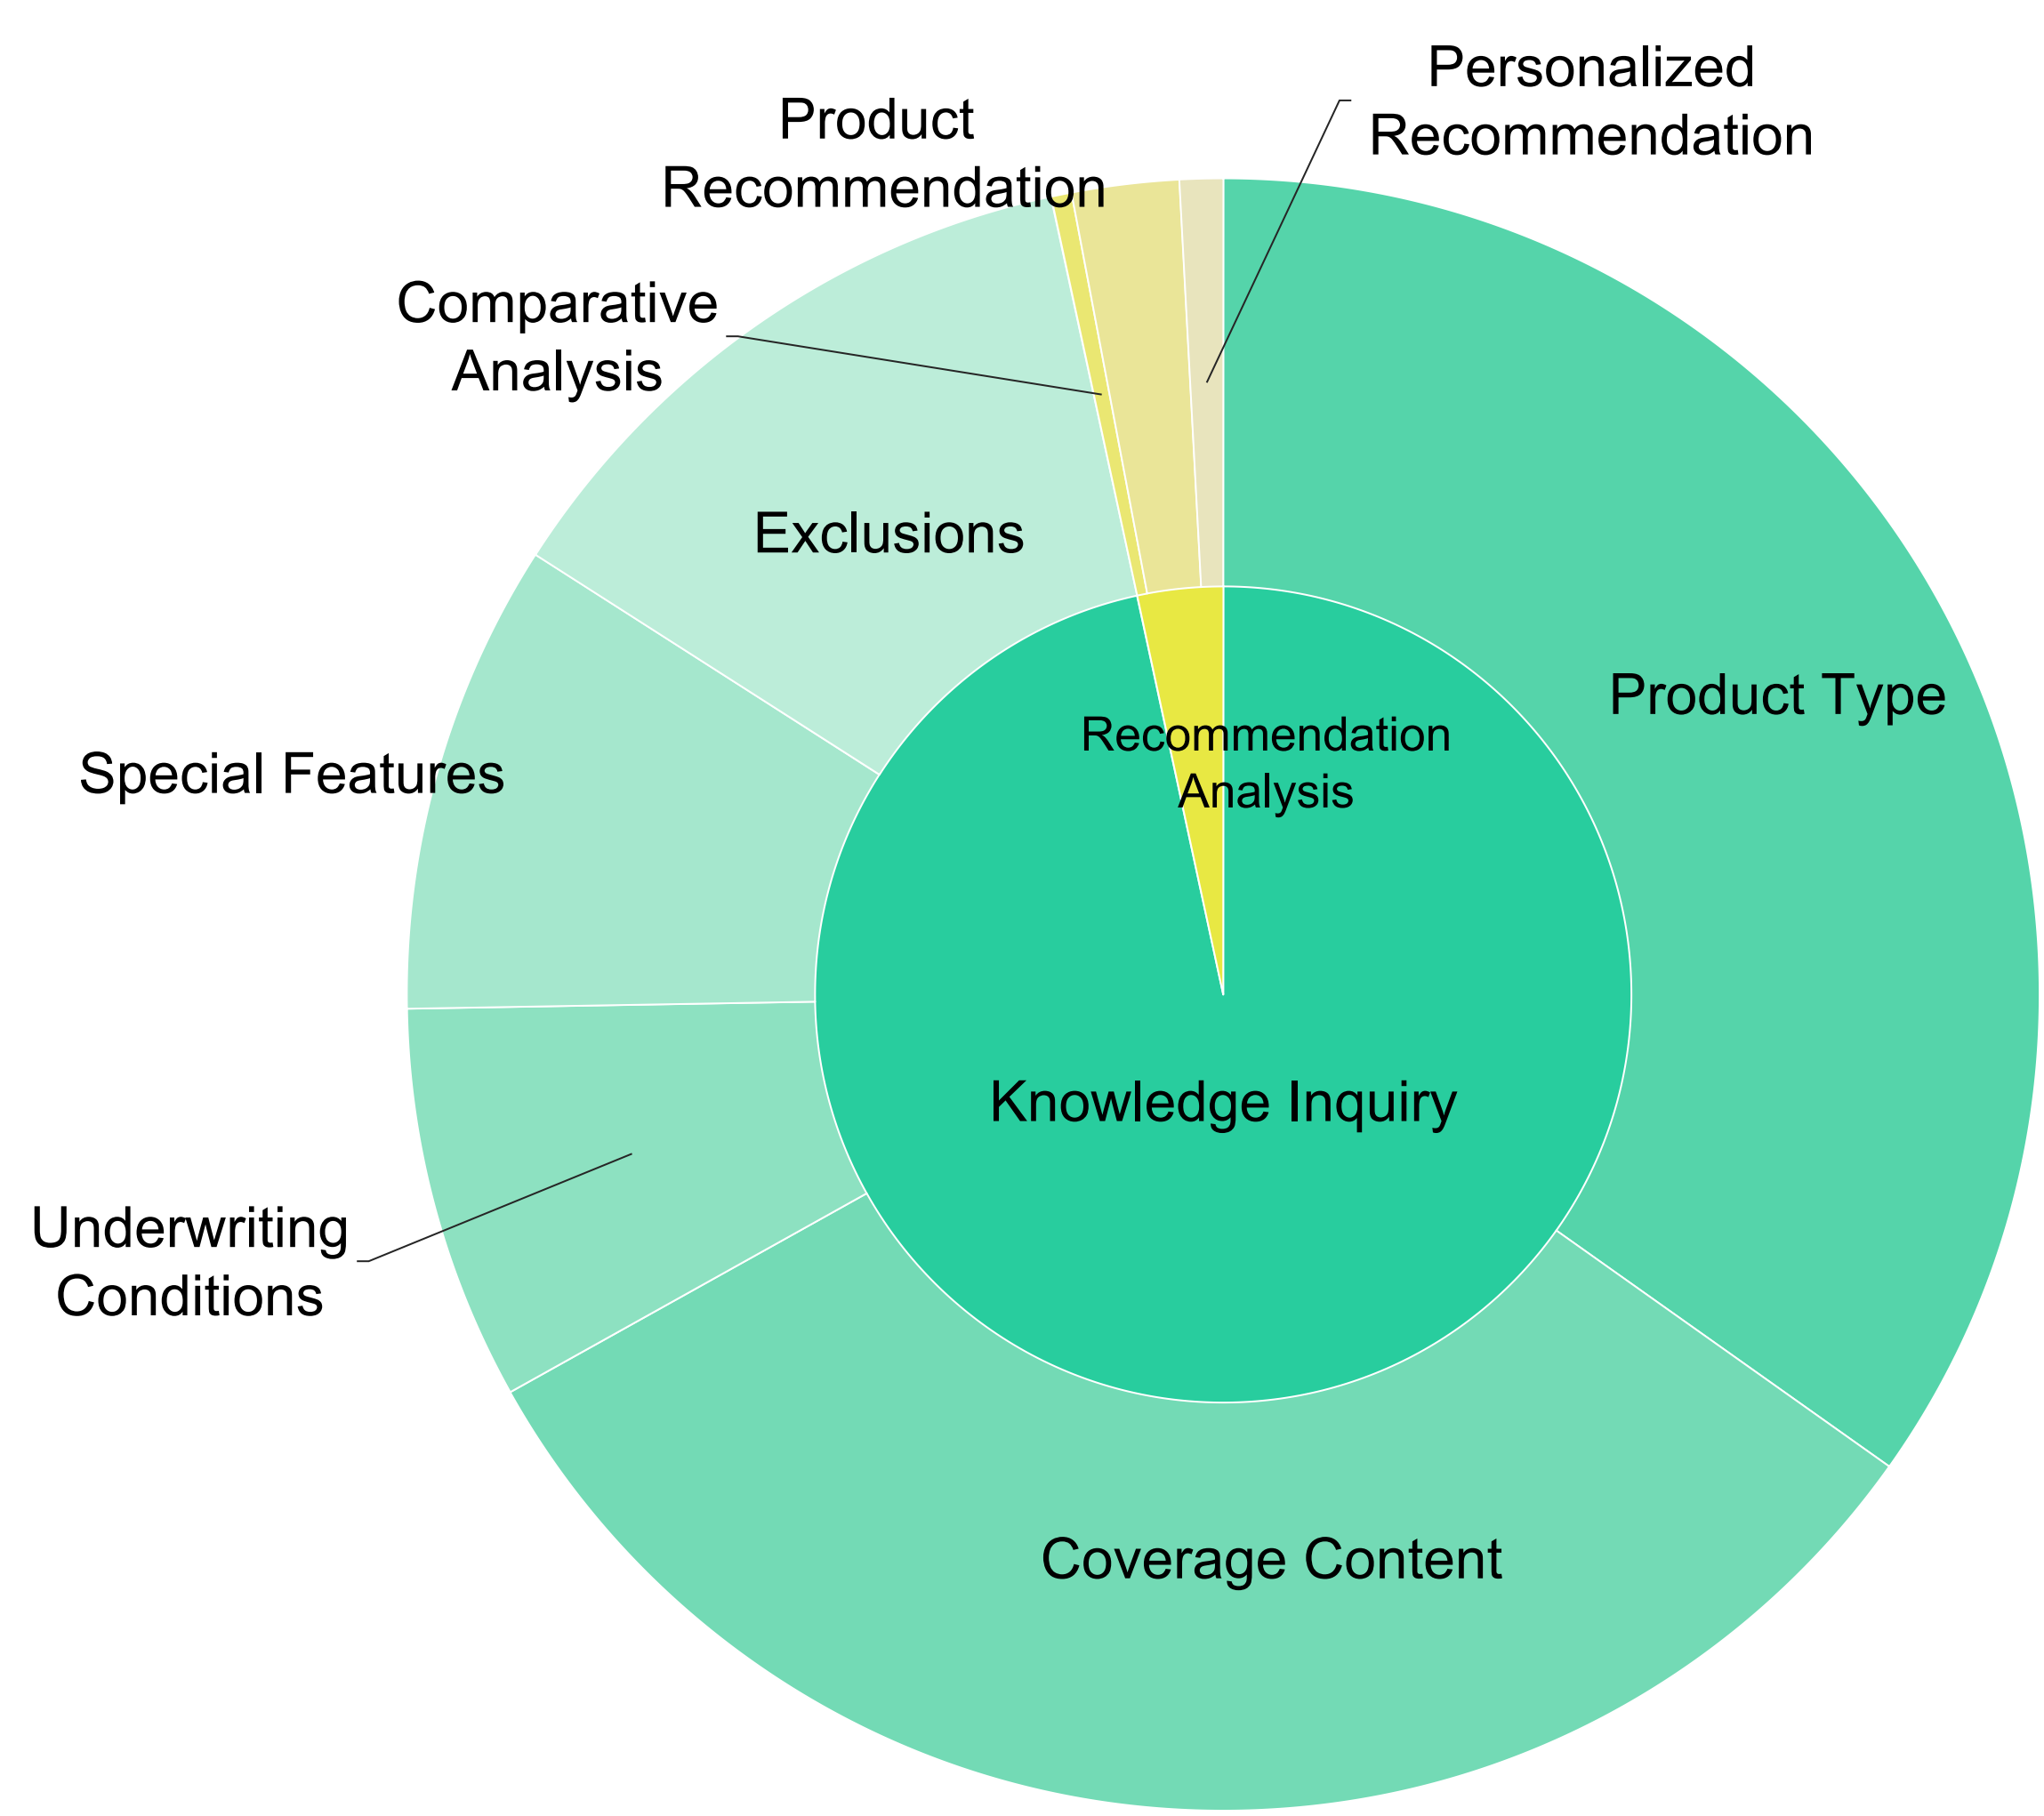

Topics in Database QA Dataset

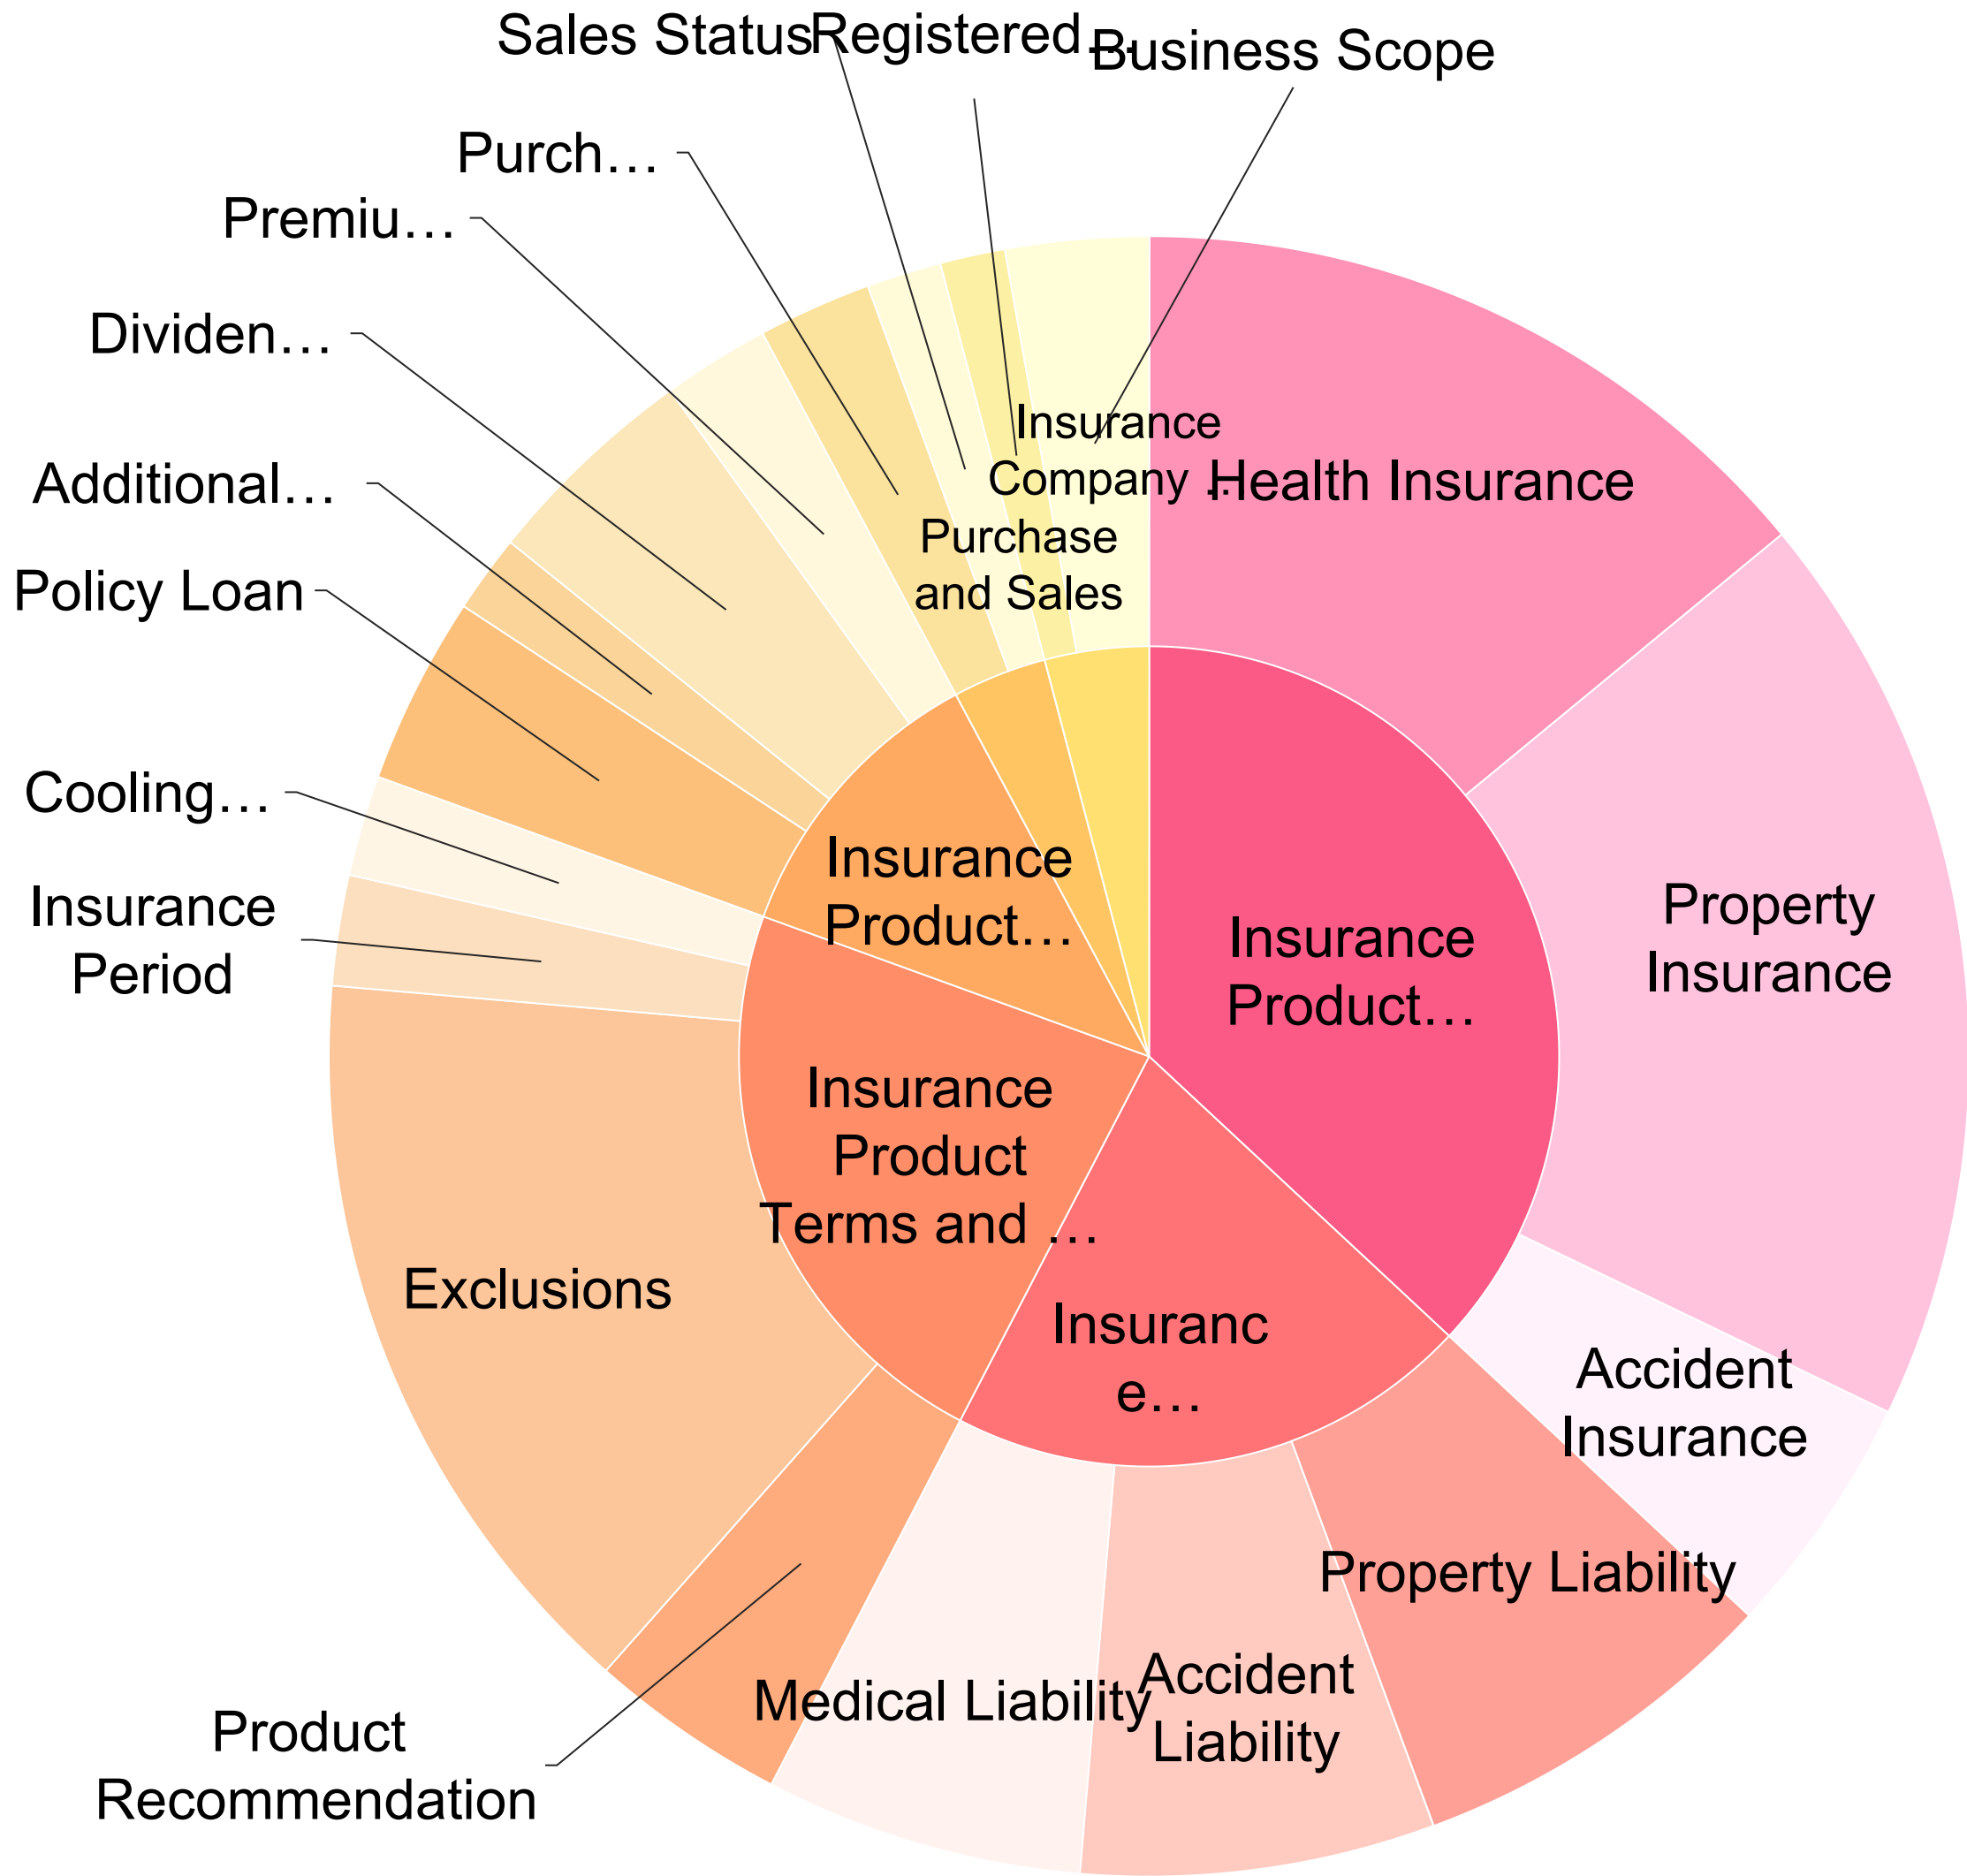

Supplement: Supplementary file 1 [file category.pdf]
